# Supplementary material for: The Entropy of Floating-Point Numbers
Source: arXiv:2605.11546 source file (2026-09-02)
Supplement: Supplementary file 1 [file approx_entropy.tex]

\section{Approximating the entropy of floating point numbers}\label{app:FPN}

Here we review the details of calculations used to approximate the entropy of floating point numbers. 









\subsubsection*{Approximation 1 -- Relating discrete and differential entropy for non-uniform bins}\label{app:FPN_app1}

Let there be a quantization scheme with $K$ representable values
$\{u_1, u_2, \ldots, u_K\}$, where $u_1 < u_2 < \cdots < u_K$.
Let $\Xv \sim f_\Xv$, where $f_\Xv$ is a differentiable probability density function with support on
\begin{equation}
\mathbb{U}^d \triangleq \left[-2^{e_{max} + 1} + 2^{e_{max} - p}, \,\, 2^{e_{max} + 1} - 2^{e_{max} - p}\right]^d,
\end{equation}
where we assume each component $X_j$ is independently clipped and quantized.

Let $\Delta: \left[-2^{e_{max} + 1} + 2^{e_{max} - p},\,\, 2^{e_{max} + 1} - 2^{e_{max} - p}\right] \to \mathbb{R}_+$
encode the bin sizes of the quantization scheme for a single component, where
\begin{equation*}
    \begin{aligned}
    \Delta(x_j) &\triangleq \sum_{i=2}^{K-1}\frac{u_{i+1} - u_{i-1}}{2}
    \indic{x_j \in \Big[\frac{u_i+u_{i-1}}{2}, \frac{u_{i+1}+u_i}{2}\Big)} + (u_2 - u_1)\indic{x_j \in [-2^{e_{max} + 1} + 2^{e_{max} - p}, \frac{u_{2} + u_{1}}{2}]}\nonumber\\
    & + (u_K - u_{K-1})\indic{x_j \in [\frac{u_{K} + u_{K-1}}{2}, 2^{e_{max} + 1} - 2^{e_{max} - p}]}.
    \end{aligned}
\end{equation*}
Since each component is stored on its own floating-point register, the quantization cell for $\Xv_Q$ is a $d$-dimensional rectangle with volume
\begin{equation}
\bDelta(\xv) \triangleq \prod_{j=1}^{d} \Delta(x_j),
\qquad
\log \bDelta(\xv) = \sum_{j=1}^{d} \log \Delta(x_j).
\end{equation}

Let $\mathbf{i} = (i_1,\dots,i_d)$ index the $d$-dimensional quantization cells, where $i_j \in \{1,\dots,K\}$. Define the cell boundaries
\begin{equation}
a_i=\begin{cases}
-2^{e_{max} + 1} + 2^{e_{max} - p} & i=1\\[2pt]
\frac{u_i+u_{i-1}}2 & 2\leq i\leq K
\end{cases},
\qquad
b_i=\begin{cases}
\frac{u_{i+1}+u_i}2 & 1\leq i\leq K-1\\[2pt]
2^{e_{max} + 1} - 2^{e_{max} - p} & i=K.
\end{cases}
\end{equation}
For each $d$-dimensional index $\mathbf{i}$, define the quantization cell
\begin{equation}
B_{\mathbf{i}} \triangleq \prod_{j=1}^d [a_{i_j}, b_{i_j}],
\end{equation}
and let
\begin{equation}
p_{\mathbf{i}} \triangleq \mathbb{P}\{\Xv\in B_{\mathbf{i}}\}
= \mathbb{P}\{\Xv_Q = \mathbf{u}_{\mathbf{i}}\},
\end{equation}
where $\mathbf{u}_{\mathbf{i}}$ is the $d$-dimensional representable value corresponding to the quantization cell $B_\mathbf{i}$.

Then the discrete entropy of $\Xv_Q$ is
\begin{equation}
H(\Xv_Q) = -\sum_{\mathbf{i}} p_{\mathbf{i}} \log p_{\mathbf{i}}.
\end{equation}

To relate this discrete entropy to the differential entropy of $\Xv$, define the piecewise-uniform density
\begin{equation}
g(\xv)
\triangleq
\sum_{\mathbf{i}}
\frac{p_{\mathbf{i}}}{|B_{\mathbf{i}}|}
\indic{\xv\in B_{\mathbf{i}}},
\label{eq:piecewise_uniform_g}
\end{equation}
where $|B_{\mathbf{i}}| = \bDelta(\xv)$ for $\xv \in B_{\mathbf{i}}$ is the volume of each rectangular cell $B_{\mathbf{i}}$. By construction, $g$ is constant on each cell and integrates to one across all cells.

Following \cite{kostina_data_2017}, we can derive an exact identity relating the discrete and differential entropies. By the definition of Kullback-Leibler divergence,
\begin{align}
\relent{f_{\Xv}}{g}
&=
\int_{\mathbb{U}^d}
f_{\Xv}(\xv)
\log\frac{f_{\Xv}(\xv)}{g(\xv)}
\,d\xv
\notag\\
&=
\int_{\mathbb{U}^d}
f_{\Xv}(\xv)\log f_{\Xv}(\xv)
\,d\xv
-
\int_{\mathbb{U}^d}
f_{\Xv}(\xv)\log g(\xv)
\,d\xv
\notag\\
&=
-h(\Xv)
-
\int_{\mathbb{U}^d}
f_{\Xv}(\xv)\log g(\xv)
\,d\xv.
\label{eq:KL_start}
\end{align}
Since $g(\xv) = p_{\mathbf{i}}/|B_{\mathbf{i}}|$ for $\xv\in B_{\mathbf{i}}$,
\begin{align}
\int_{\mathbb{U}^d}
f_{\Xv}(\xv)\log g(\xv)
\,d\xv
&=
\sum_{\mathbf{i}}
\int_{B_{\mathbf{i}}}
f_{\Xv}(\xv)
\log\left(\frac{p_{\mathbf{i}}}{|B_{\mathbf{i}}|}\right)
d\xv\\
&=
\sum_{\mathbf{i}}
 \bigg(
\int_{B_{\mathbf{i}}}
f_{\Xv}(\xv) d\xv\bigg)
\log\left(\frac{p_{\mathbf{i}}}{|B_{\mathbf{i}}|}\right)
=
\sum_{\mathbf{i}}
p_{\mathbf{i}}
\log\left(\frac{p_{\mathbf{i}}}{|B_{\mathbf{i}}|}\right)\\
&=
\sum_{\mathbf{i}} p_{\mathbf{i}}\log p_{\mathbf{i}}
-
\sum_{\mathbf{i}} p_{\mathbf{i}}\log |B_{\mathbf{i}}|.
\label{eq:KL_middle}
\end{align}
Substituting Eq.~\eqref{eq:KL_middle} into Eq.~\eqref{eq:KL_start} yields
\begin{align}
\relent{f_{\Xv}}{g}
&=
-h(\Xv)
-
\sum_{\mathbf{i}} p_{\mathbf{i}}\log p_{\mathbf{i}}
+
\sum_{\mathbf{i}} p_{\mathbf{i}}\log |B_{\mathbf{i}}|
\notag\\
&=
-h(\Xv)
+
H(\Xv_Q)
+
\mathbb{E}[\log \bDelta(\Xv)],
\end{align}
or equivalently,
\begin{equation}
H(\Xv_Q)
=
h(\Xv)
-
\mathbb{E}[\log \bDelta(\Xv)]
+
\relent{f_{\Xv}}{g}.
\label{eq:exact_identity}
\end{equation}
Approximation 1 corresponds to neglecting the nonnegative correction term $\relent{f_{\Xv}}{g}$:
\begin{equation}
H(\Xv_Q)
\approx
h(\Xv)
-
\mathbb{E}[\log \bDelta(\Xv)].
\label{eq:approx1_clean}
\end{equation}

\cite{kostina_data_2017} shows rigorously that the correction term $\relent{f_{\Xv}}{g}$ becomes large if $f_{\Xv}$ varies noticeably within each quantization cell, and vanishes if the function is uniform across each cell. Here, we can understand this at a basic level by noting that $g(\xv)$ is equal to the mean value of $f_{\Xv}$ within a given bin $B_{\mathbf{i}}$. By the multivariate mean value theorem, $g(\xv) = f_\Xv(\mathbf{\tilde x_{\mathbf{i}}})$ for some $\mathbf{\tilde x}_{\mathbf{i}} \in B_{\mathbf{i}}$. Taylor expanding $f_{\Xv}(\xv)$ within cell $B_{\mathbf{i}}$ to first order around $\mathbf{\tilde x}_{\mathbf{i}}$ we see:
\begin{equation}
f_{\Xv}(\xv) \approx g (\xv)+ \nabla f_{\Xv}(\mathbf{\tilde x}_{\mathbf{i}}) \cdot (\xv- \mathbf{\tilde x}_{\mathbf{i}}).
\end{equation}
Since $\relent{f_{\Xv}}{g} \approx 0$ when $f_{\Xv} \approx g$, a cell can contribute significantly to the error if the size of the cell and the gradient of $f_{\Xv}$ are simultaneously large, since $(\xv-\mathbf{\tilde x}_{\mathbf{i}})$ is bounded by the size of the cell. However, when the cell diameter is small in regions where the density varies rapidly, or if the cell diameter is large where the density varies only slowly, the discrepancy between $f_{\Xv}$ and its cell average $g(\xv)$ remains small.

Finally, we can note that if each component is quantized independently, then
\begin{equation}
\mathbb{E}[\log \bDelta(\Xv)]
=
\sum_{j=1}^{d}\mathbb{E}_{X_j}[\log \Delta(X_j)],
\label{eq:separable}
\end{equation}
so that Approximation 1 takes the form
\begin{equation}
\tilde{H}(\Xv_Q)
\triangleq
h(\Xv)
-
\sum_{j=1}^{d}\mathbb{E}_{X_j}[\log \Delta(X_j)].
\label{eq:multi_var_diff_disc}
\end{equation}










\subsubsection*{Approximation 2 -- Smoothing the bin size function and extending its domain}\label{app:FPN_app2}

In the multivariate case, with $\Delta_s(x) = \frac{|x|}{\sqrt{2}}\cdot 2^{1-p}$ from Eq.~\eqref{eq:step_approx}, we can define
\begin{equation}
    \bDeltas(\xv) = \prod^d_{j=1} \Delta_s(x_j).
\end{equation}
Again, $\mathbb{U}^d = [-2^{e_{max} + 1} + 2^{e_{max} - p}, \,\, 2^{e_{max} + 1} - 2^{e_{max} - p}]^d$, where $e_{max} = 2^{E-1}$. Assuming that the tails of $f_\Xv$ are vanishingly small,
\begin{equation}
    \int_{\mathbb{R}^d \setminus \mathbb{U}^d} f_\Xv(\xv) \, d\xv \approx 0,
\end{equation}
we extend the domain from $\mathbb{U}^d$ to $\mathbb{R}^d$. As noted in the main text, this extension requires that the omitted tail integral $\int_{\mathbb{R}^d\setminus\mathbb{U}^d} f_\Xv(\xv)|\log[f_\Xv(\xv)\bDeltas(\xv)]|\,d\xv$ is near zero, not merely that the tail mass is small. For the Gaussian and Student's $t$ distributions used in this paper, the tail decay dominates the linear growth of $\Delta_s$, so this tail integral is negligible when the granular region $\mathbb{U}$ is sufficiently large (i.e., $E$ is not too small). With this we can say from Eq.~\eqref{eq:multi_var_diff_disc} $\tilde H(\Xv_Q) \approx \tilde H_s(\Xv_Q)$, where
\begin{equation}
    \tilde H_s(\Xv_Q) = -\int_{\mathbb{R}^d}  f_\Xv(\xv)
    \log\left[f_\Xv(\xv)
    \prod_{j=1}^d \Delta_s(x_j)\right] d\xv.
\end{equation}













Define the smooth-bin approximation restricted to $\mathbb U^d$ as
\begin{equation}
\label{eq:Ht_s_U}
\tilde H_{s,\mathbb U}(\Xv_{fp})
\;\triangleq\;
-\int_{\mathbb U^d} f_{\Xv}(\xv)\,\log\left[f_{\Xv}(\xv)\prod_{j=1}^d \Delta_s(x_j)\right]d\xv.
\end{equation}
Theorem~\ref{thm:steps} bounds the smoothing error by the $d/2$ term plus the explicit contribution from the bins adjacent to zero.

Define the special-bin set
\begin{equation}
\label{eq:special_bins}
\begin{aligned}
\mathcal B_0 &\triangleq \left\{x\in \mathbb U:\ |x|<2^{e_{\min}}(1+2^{-p})\right\}
\end{aligned}
\end{equation}
where $\mathcal B_0$ is the union of the two bins adjacent to $0$. When $x \in \mathcal B_{0}$, $\Delta(x) = \Delta_0 = 2^{e_{\min}}(1+2^{-p})$. Define
\begin{equation}
\label{eq:special_error}
\varepsilon_{0}(\Xv)
\triangleq
\sum_{j=1}^{d}
\int_{\mathcal B_{0}}
f_{X_j}(x)
\left|
\log\bracket{\frac{\Delta_s(x)}{\Delta_0}}
\right|dx.
\end{equation}

\begin{theorem}[Error bound for smoothing the bin-size function]\label{thm:steps}
Let $\Xv\sim f$ be a $d$-dimensional random vector with the probability density $f$ supported on $\mathbb U^d$, and let $X_j$ denote its $j$th component. Let $\tilde H(\Xv_{fp})$ be the approximation from App.~\ref{app:FPN_app1} using the true midpoint bin-size function $\Delta$, and let $\tilde H_{s,\mathbb U}(\Xv_{fp})$ be the corresponding approximation on $\mathbb U^d$ using $\Delta_s$. Then
\begin{equation}
\abs{\tilde H(\Xv_{fp}) - \tilde H_{s,\mathbb U}(\Xv_{fp})} \leq \frac{d}{2} + \varepsilon_{0}(\Xv),
\end{equation}
where $\varepsilon_{0}(\Xv)$ is finite and defined in Eq.~\eqref{eq:special_error}.
\end{theorem}

\begin{proof}

There are 3 types of bins for which we will bound the error: bins on the interior of an exponent block, bins on the outer edges, and bins on the boundary between exponent blocks (regions for which a single exponent value applies). The bound can be shown by considering the ratio between bin sizes, case by case.

\paragraph{Interior Bins}
For interior bins strictly within each exponent block $e$, by Eq.~\eqref{eq:true_bins},
\begin{equation}
    \label{eq:real_bins}
    \Delta(x_j) = 2^{e-(p-1)} \quad \text{for } 2^e \leq |x_j| < 2^{e+1},
\end{equation}
and within this range $\Delta_s(x_j) = \frac{|x_j|}{\sqrt{2}} \cdot 2^{1-p}$ satisfies
\begin{equation}
    \begin{aligned}
    &\frac{2^e}{\sqrt{2}}2^{1-p} \leq \Delta_s(x_j) \leq \frac{2^{e+1}}{\sqrt{2}}2^{1-p}\\
    \implies &\frac{1}{\sqrt{2}} \leq \frac{\Delta_s(x_j)}{\Delta(x_j)} < \sqrt{2}.
    \end{aligned}
\end{equation}

\paragraph{Outer clipping bins}

For the outer clipping bins, by symmetry it suffices to analyze $[\frac{u_K + u_{K-1}}{2}, 2^{e_{\max}+1}-2^{e_{\max}-p}]$ which is the bin on positive side of the real line. When $p \geq 2$, we know that $u_K = 2^{e_{max}+1}(1 - 2^{-p})$, and $u_{K-1} = 2^{e_{max}+1}(1 - 2^{1-p})$, so the outer clipping bin size is \begin{equation}
\Delta(x_j) = 2^{e_{max} + 1} - 2^{e_{max} - p}- \frac{u_K + u_{K-1}}{2} = 2^{e_{max}}\paren{2^{1-p}} = 2^{e_{max}-p + 1}
\end{equation}
Now, we have
\begin{equation}
\begin{aligned}
  &\frac{(u_K + u_{K-1})}{2\sqrt{2}}2^{1-p} \leq \Delta_s(x_j) \leq \frac{2^{e_{max} + 1} - 2^{e_{max} - p}}{\sqrt{2}}2^{1-p}\\
  \implies &\frac{ 2^{e_{max}}(1 - 2^{-1-p} - 2^{-p})}{2^{e_{max} - p}\sqrt{2}}2^{1-p} \leq \frac{\Delta_s(x_j)}{\Delta(x_j)} \leq \frac{2^{e_{max}}(1 - 2^{-1 - p})}{2^{e_{max} - p}\sqrt{2}}2^{1-p}\\
  \implies &\frac{ 2(1 - 2^{-1-p} - 2^{-p})}{\sqrt{2}} \leq \frac{\Delta_s(x_j)}{\Delta(x_j)} \leq \frac{2(1- 2^{-1-p})}{\sqrt{2}}\\
  \implies &\sqrt{2}(1 - 2^{-1-p} - 2^{-p}) \leq \frac{\Delta_s(x_j)}{\Delta(x_j)} \leq \sqrt{2}(1- 2^{-1-p}).
\end{aligned}
\end{equation}
When $p = 1$, $u_K = 2^{e_{max}}$ and $u_{K-1} = 2^{e_{max}-1}$. The true bin width is 
\begin{equation}
\Delta(x_j) = 2^{e_{max}+1} - 2^{e_{max}-1} - \frac{1}{2}(2^{e_{max}} + 2^{e_{max}-1}) = 3\cdot2^{e_{max}-2}.
\end{equation}
Using the same bounding technique, we have
\begin{equation}
\begin{aligned}
  &\frac{2^{e_{max}} + 2^{e_{max}-1}}{2\sqrt{2}} \leq \Delta_s(x_j) \leq \frac{2^{e_{max}+1} - 2^{e_{max}-1}}{\sqrt{2}}\\
  \implies &\frac{3\cdot 2^{e_{max}-2}}{3\cdot2^{e_{max}-2}\sqrt{2}} \leq \frac{\Delta_s(x_j)}{\Delta(x_j)} \leq \frac{3\cdot 2^{e_{max}-1}}{3\cdot2^{e_{max}-2}\sqrt{2}}\\
  \implies &\frac{ 1}{\sqrt{2}} \leq \frac{\Delta_s(x_j)}{\Delta(x_j)} \leq \frac{2}{\sqrt{2}}.
\end{aligned}
\end{equation}
For the outer clipping bins, we see that for all $p\geq 1$, $\frac{1}{\sqrt{2}} \leq \frac{\Delta_s(x_j)}{\Delta(x_j)} \leq \sqrt{2}$.

\paragraph{Exponent boundary bins}

At exponent boundaries, let the last representable value of the $e$-th exponent block be $u_A = 2^{e+1} - 2^{e-(p-1)}$. the first representable value of the $e+1$-th exponent block be $u_B = 2^{e+1}$, and the second representable value of the $e+1$-th exponent block be $u_C = 2^{e+1} + 2^{e+1 - (p-1)}$. The left boundary of the midpoint-quantization bin for $u_B$ is $m_L = \frac{u_A + u_B}{2} = 2^{e+1}(1 - 2^{-p-1})$ while the right boundary is $m_R = \frac{u_B + u_C}{2} = 2^{e+1}(1+2^{-p})$. When $x_j \in [m_L, m_R)$, the bin width is
\begin{equation}\label{eq:exp_boundary}
\Delta(x_j) = m_R - m_L = 3 \cdot 2^{e-p},
\end{equation}
and the ratio $\Delta_s(x_j)/\Delta(x_j)$ is bounded by
\begin{equation}
    \begin{aligned}
    &\frac{2^{e+1}(1 - 2^{-p-1})}{\sqrt{2}}2^{1-p} \leq \Delta_s(x_j) \leq \frac{2^{e+1}(1+2^{-p})}{\sqrt{2}}2^{1-p}\\
    \implies & \frac{2^{e+1}(1 - 2^{-p-1})}{3 \cdot 2^{e-p}\sqrt{2}}2^{1-p} \leq \frac{\Delta_s(x_j)}{\Delta(x_j)} \leq \frac{2^{e+1}(1+2^{-p})}{3 \cdot 2^{e-p}\sqrt{2}}2^{1-p}\\
    \implies & \frac{2\sqrt{2}(1 - 2^{-p-1})}{3} \leq \frac{\Delta_s(x_j)}{\Delta(x_j)}  \leq \frac{2\sqrt{2}(1+2^{-p})}{3}.
    \end{aligned}
\end{equation}
When $p = 1$ the lower bound is equal to $1/\sqrt{2}$ and the upper bound is equal to $\sqrt{2}$. The lower bound is monotonically increasing in $p$ while the upper bound is monotonically decreasing in $p$, and both converge to $2\sqrt{2}/3$ as $p \rightarrow \infty$, which is between $1/\sqrt{2}$ and $\sqrt{2}$. This means both bounds lie within $[1/\sqrt{2},\, \sqrt{2}]$, so for within exponent block bins and exponent boundary bins,
\begin{equation}
    -\frac{1}{2} \leq \log\left[\frac{\Delta_s(x_j)}{\Delta(x_j)}\right] < \frac{1}{2}.
\end{equation}

\paragraph{Bound on entropy difference from bin ratios}


Hence, for every $x_j\in \mathbb U\setminus \mathcal B_{0}$,
\begin{equation}
\abs{\log\bracket{\frac{\Delta_s(x_j)}{\Delta(x_j)}}} \leq \frac{1}{2}.
\end{equation}

The remaining points are exactly the special bins collected in $\mathcal B_{0}$, where we do not claim a uniform pointwise bound and instead keep their contribution explicitly:
\begin{equation}
\begin{aligned}
&\left|
\tilde H(\Xv_{fp}) - \tilde H_{s,\mathbb U}(\Xv_{fp}) \right| = \Bigg | -\int_{\mathbb U^d} f_{\Xv}(\xv)\,\log\left[f_{\Xv}(\xv)\prod_{j=1}^d \Delta(x_j)\right]d\xv  \\ & \qquad \qquad \qquad \qquad \qquad
+ \int_{\mathbb U^d} f_{\Xv}(\xv)\,\log\left[f_{\Xv}(\xv)\prod_{j=1}^d \Delta_s(x_j)\right]d\xv \Bigg |\\
&\left|
\tilde H(\Xv_{fp}) - \tilde H_{s,\mathbb U}(\Xv_{fp}) \right| = \abs{\sum_{j=1}^{d} \Esub{\log\bracket{\frac{\Delta_s(x)}{\Delta(x)}}}{X_j}} \\
&\leq\sum_{j=1}^{d} \int_{\mathbb U\setminus \mathcal B_{0}} f_{X_j}(x) \abs{\log\bracket{\frac{\Delta_s(x)}{\Delta(x)}}}dx + \varepsilon_{0}(\Xv) \leq\frac d2 + \varepsilon_{0}(\Xv).
\end{aligned}
\end{equation}
The point $x=0$ has measure zero, and $\varepsilon_{0}(\Xv)$ is finite since each marginal density is continuous on $\mathbb U$ while $|\log|x||$ is locally integrable near $0$.
\end{proof}

Not only is $\varepsilon_{0}(\Xv)$ finite, as shown in Theorem~\ref{thm:steps}, but for the probability distributions that this paper studies, Corollary~\ref{cor:eps_sp_bound} shows that $\varepsilon_{0}(\Xv)$ is negligibly small.


\begin{corollary}[Bound on $\varepsilon_{0}$ for densities bounded near zero]
\label{cor:eps_sp_bound}
Under the hypotheses of Theorem~\ref{thm:steps}, with
$\mathcal{B}_{0} = \mathcal{B}_0$ (the two zero-crossing bins),
define
\begin{equation}
  a \;\triangleq\; 2^{e_{\min}}\bigl(1 + 2^{-p}\bigr),
  \qquad
  C_0 \;\triangleq\; 2\,a\left(p - \frac{1}{2} + \log e\right).
\end{equation}
Then
\begin{equation}
\label{eq:eps_sp_general}
  \varepsilon_{0}(\Xv)
  \;\le\;
  C_0
  \sum_{j=1}^{d}
  \sup_{x \in \mathcal{B}_0} f_{X_j}(x).
\end{equation}
 
If every marginal density $f_{X_j}$ attains its mode at $0$,
then
\begin{equation}
\label{eq:eps_sp_mode}
  \varepsilon_{0}(\Xv)
  \;\le\;
  C_0
  \sum_{j=1}^{d} f_{X_j}(0).
\end{equation}
 
\medskip
\noindent\textbf{(i)\; Zero-mean Gaussian marginals.}\;
If $X_j \sim \mathcal{N}(0,\sigma_j^2)$, then $f_{X_j}(0) = 1/(\sigma_j\sqrt{2\pi})$, and
\begin{equation}
\label{eq:eps_sp_gauss}
  \varepsilon_{0}(\Xv)
  \;\le\;
  \frac{C_0}{\sqrt{2\pi}}
  \sum_{j=1}^{d} \frac{1}{\sigma_j}.
\end{equation}
 
\noindent\textbf{(ii)\; Scaled Student's $t$ marginals.}\;
If $X_j \sim t_\nu(0,\sigma_j)$ with density
$f_{X_j}(x)
= \frac{\Gamma\bigl(\frac{\nu+1}{2}\bigr)}
       {\sigma_j\sqrt{\nu\pi}\;\Gamma\bigl(\frac{\nu}{2}\bigr)}
  \bigl(1 + x^2/(\nu\sigma_j^2)\bigr)^{-(\nu+1)/2}$,
then $f_{X_j}(0) = \Gamma\bigl(\frac{\nu+1}{2}\bigr)
  \big/\bigl(\sigma_j\sqrt{\nu\pi}\;\Gamma\bigl(\frac{\nu}{2}\bigr)\bigr)$, and
\begin{equation}
\label{eq:eps_sp_student}
  \varepsilon_{0}(\Xv)
  \;\leq\;
  \frac{C_0\;\Gamma\bigl(\frac{\nu+1}{2}\bigr)}
       {\sqrt{\nu\pi}\;\Gamma\bigl(\frac{\nu}{2}\bigr)}
  \sum_{j=1}^{d} \frac{1}{\sigma_j}.
\end{equation}
\end{corollary}
 
\begin{proof}
We see that $a$ is the value of the first interior midpoint for positive bin adjacent to zero $(0, a]$. The true midpoint bin width is,
$\Delta(x_j) = a$,
while $\Delta_s(x_j) = x \cdot 2^{1-p}/\sqrt{2}$.
Since on this interval $x_j 2^{1-p}/\sqrt{2} \leq x_j \leq a$, the ratio $\Delta_s(x_j)/\Delta(x_j) < 1$
on the entire bin, so
\begin{equation}
  \abs{\log\bracket{\Delta_s(x)/\Delta(x)}}
  = \log\bracket{\frac{a \cdot 2^{p-1/2}}{x}}.
\end{equation}
By symmetry the negative bin $[-a, 0)$ gives the same integrand in $|x|$.
Therefore, for each marginal,
\begin{align}
  \int_{\mathcal{B}_0} f_{X_j}(x)
    \bigl|\log\bracket{\Delta_s(x)/\Delta(x)}\bigr|\,dx
  &\leq
  \sup_{t \in \mathcal{B}_0} f_{X_j}(t)
  \;\cdot\;
  2\int_0^{a} \log\bracket{\frac{a\cdot 2^{p-1/2}}{x}}dx.
\end{align}
The integral evaluates as
\begin{align}
  2\int_0^{a} \log\bracket{\frac{a\cdot 2^{p-1/2}}{x}}dx
  &= 2\int_0^{a}\Bigl[\bigl(p - \frac{1}{2}\bigr)
     + \log[a/x]\Bigr]dx \notag\\
  &= 2a\left(p - \frac{1}{2}\right)
     + \frac{2}{\ln 2}\int_0^{a}\ln[a/x]\,dx \notag\\
  &= 2a\left(p - \frac{1}{2}\right) + \frac{2a}{\ln 2}
  \;=\; 2a\left(p - \frac{1}{2} + \log e\right)
  \;=\; C_0,
\end{align}
where we used $\int_0^{a}\ln[a/x]\,dx = a$.
Summing over $j=1,\dots,d$ gives Eq.~\eqref{eq:eps_sp_general}.

When each $f_{X_j}$ has its mode at zero,
$\sup_{x\in\mathcal{B}_0} f_{X_j}(x) = f_{X_j}(0)$,
yielding Eq.~\eqref{eq:eps_sp_mode}.
Substituting $f_{X_j}(0)$ for $\mathcal{N}(0,\sigma_j^2)$ and
$t_\nu(0,\sigma_j)$ gives Eqs.~\eqref{eq:eps_sp_gauss}
and~\eqref{eq:eps_sp_student}.
\end{proof}
 
For candidate floating-point formats and identical marginals
($\sigma_j = \sigma$ for all $j$), Figure~\ref{fig:eps0_C0_vs_p}
shows $C_0$ and the per-dimension bound $\varepsilon_{0}/d$
as functions of the precision $p$ for several exponent widths $E$,
with $\sigma = 1$ and $d = 1$.
Gaussian marginals are shown as circles and
Student's $t_5$ marginals as squares; the two nearly overlap because
the ratio
$\Gamma\bigl(\frac{\nu+1}{2}\bigr)\sqrt{2/\nu}\big/\Gamma\bigl(\frac{\nu}{2}\bigr)$
is $O(1)$ for all $\nu \ge 1$.
By $E = 4$, $\varepsilon_0 \approx 0.16$ for $p = 24$. 

\begin{figure}[htbp]
  \centering
  \begin{subfigure}[t]{0.48\textwidth}
    \centering
    \includegraphics[width=\textwidth]{code/quantized_entropy_midpoint/C0_vs_p.pdf}
    \caption{$C_0$ vs.\ precision $p$.}
    \label{fig:C0_vs_p}
  \end{subfigure}
  \hfill
  \begin{subfigure}[t]{0.48\textwidth}
    \centering
    \includegraphics[width=\textwidth]{code/quantized_entropy_midpoint/eps0_vs_p.pdf}
    \caption{$\varepsilon_{0}$ bound vs.\ precision $p$.}
    \label{fig:eps0_vs_p}
  \end{subfigure}
  \caption{Numerical scale of $C_0$ and $\varepsilon_{0}$ (Corollary~\ref{cor:eps_sp_bound}) for $d=1$, $\sigma=1$.
  Each curve corresponds to a different exponent width $E$.
  Circles denote Gaussian marginals; squares denote Student's $t_5$ marginals.}
  \label{fig:eps0_C0_vs_p}
\end{figure}

\FloatBarrier
% \subsubsection*{Approximation 3 -- $\mathbb{E}[\log[|x|/\sqrt{2}]]$}\label{app:FPN_app3}

% \begin{figure}[htbp]
%   \centering
%     \includegraphics[trim={1cm 0.0cm 16cm 0.85cm}, clip,width=0.5\textwidth]{code/quantized_entropy_midpoint/entropy_vs_mu_all_approx.pdf}
% \caption{\textit{Simulating approximation 3: }  The dependence of the entropy of a normally distributed floating-point number on its standard deviation $\sigma$ and mean $\mu$. Dashed lines show Approximation 3 from Eq.~\eqref{eq:three_approxes}, while solid lines show the exact entropy from Corollary~\ref{cor:gauss_fp_ent}.}\label{fig:fp_off_zero}
% \end{figure}

% We can show that Eq.~\eqref{eq:first_two_approx} approximates Eq.~\eqref{eq:three_approxes} in two cases. First, for a Gaussian distribution where its mean is significantly greater than its standard deviation, $\mu \gg \sigma$. Second, for a distribution $X \sim f_{X}(x,\epsilon)$ that approximates a Dirac delta function as $\epsilon \rightarrow 0$. 

% \textit{Non-zero mean Gaussian: }First, for a non-zero mean Gaussian, let $X = \mu + \epsilon$ where $\epsilon \sim \mathcal{N}(0, \sigma^2)$. Without loss of generality, assume $\mu > 0$ (the final result depends only on $|\mu|$). $\log\bracket{\abs{X/\sqrt{2}}}$ becomes\begin{align}
%     \log\left|\frac{X}{\sqrt{2}}\right| = \log\left|\frac{\mu + \epsilon}{\sqrt{2}}\right| 
%     = \log\left|\frac{\mu}{\sqrt{2}}\left(1 + \frac{\epsilon}{\mu}\right)\right| 
%     = \log\left|\frac{\mu}{\sqrt{2}}\right| + \log\left|1 + \frac{\epsilon}{\mu}\right|.\label{eq:split_x}
% \end{align}
% To control the second term, we can split according to the events
% \begin{equation}
%     A=\left\{\abs{\frac{\epsilon}{\mu}} \leq \frac{1}{2}\right\} = \left\{X \in \bracket{\frac{\mu}{2}, \frac{3\mu}{2}}\right\}, \qquad A^c= \left\{|\frac{\epsilon}{\mu}| > \frac{1}{2}\right\}.
% \end{equation}
% Events in $A^c$ are exponentially unlikely when $\mu\gg\sigma$, since $P(A^c)$ is equal to
% \begin{align}
%     \mathbb P(A^c)& =\int_{-\infty}^{-\mu/2} \frac{\exp[-t^2/2\sigma^2]}{\sigma \sqrt{2\pi}} dt + \int_{\mu/2}^{\infty} \frac{\exp[-t^2/2\sigma^2]}{\sigma\sqrt{2\pi}}\,dt  = 2 \int_{\mu/2}^{\infty} \frac{\exp[-t^2/2\sigma^2]}{\sigma\sqrt{2\pi}}\,dt. \\
%     &= 2\int_{\mu/2}^{\infty} \frac{\sigma}{t} \cdot
%        \frac{t}{\sigma^2} \cdot
%        \frac{\exp[-t^2/2\sigma^2]}{\sqrt{2\pi}}\,dt \leq \frac{4\sigma}{\mu} \int_{\mu/2}^{\infty}
%        \frac{t}{\sigma^2} \cdot
%        \frac{\exp[-t^2/2\sigma^2]}{\sqrt{2\pi}}\,dt \\
%     & = \frac{4\sigma}{\mu\sqrt{2\pi}}\left[-\exp\left[-\frac{t^2}{2\sigma^2}
%        \right]\right]_{\mu/2}^{\infty} = \frac{4\sigma}{\mu\sqrt{2\pi}}\,e^{-\mu^2/(8\sigma^2)}\label{eq:p_ac_bound}
% \end{align}
% meaning that for $\mu \gg \sigma$, $P(A^c)$ is small.

% By the law of total expectation,
% \begin{equation}\label{eq:total_expect}
%     \mathbb{E}\left[\log\left|1 + \frac{\epsilon}{\mu}\right|\right] = \mathbb{E}\left[\log\left|1 + \frac{\epsilon}{\mu}\right|\,\middle|\, A\right]P(A) + \mathbb{E}\left[\log\left|1 + \frac{\epsilon}{\mu}\right|\,\middle|\, A^c\right]P(A^c).
% \end{equation}
% For the first term, on $A$ we have $1+\epsilon/\mu > 0$, so the Mercator series converges:
% \begin{equation}
%     \log\left[1 + \frac{\epsilon}{\mu}\right] = \frac{1}{\ln[2]} \left( \frac{\epsilon}{\mu} - \frac{\epsilon^2}{2\mu^2} + O \left (\frac{\epsilon^3}{\mu^3}\right ) \right).
% \end{equation}
% Since $1+\epsilon/\mu > 0$ on $A$, the absolute value can be dropped. On $A = \{|\epsilon/\mu| \le 1/2\}$, the Mercator remainder satisfies $|\ln[1+x] - x + x^2/2| \le \frac{2}{3}|x|^3$ for $|x| \le 1/2$. Therefore,
% \begin{equation}
%     \E{\left|\ln\left(1+\frac{\epsilon}{\mu}\right) - \frac{\epsilon}{\mu} + \frac{\epsilon^2}{2\mu^2}\right| \Bigg|A} \le \frac{2}{3}\frac{\E{|\epsilon|^3|A}}{|\mu|^3} = O\left(\frac{\sigma^3}{\mu^3}\right).
% \end{equation}
% $\mathbb{E}[\epsilon \mid A] = 0$ since the distribution of $\epsilon$ is symmetric over the interval $\bracket{-\mu/2, \, \mu/2}$ and by the monotone convergence theorem as $\mu/\sigma \to \infty$,  $\mathbb{E}[\epsilon^2 \mid A] \to \sigma^2$. Thus,
% \begin{equation}
%     \mathbb{E}\left[\log\left|1 + \frac{\epsilon}{\mu}\right|\,\middle|\, A\right]P(A) = \frac{P(A)}{\ln[2]} \left( - \frac{\sigma^2}{2\mu^2} + O\left(\frac{\sigma^3}{|\mu|^3}\right) \right) \approx -\frac{\sigma^2}{2\mu^2 \ln[2]}.
% \end{equation}

% For the term pertaining to $A^c$, Lemma~\ref{lem:Ac-bound} shows that $\mathbb{E}\left[\left|\log\left|1 + \epsilon/\mu\right|\right|\,\middle|\, A^c\right]\mathbb{P}(A^c) \to 0$ as $\mu/\sigma \to \infty$, which means taking the expectation of Eq.~\eqref{eq:split_x} gives
% \begin{equation}
%     \mathbb{E} \left[\log\left|\frac{X}{\sqrt{2}}\right| \right] \approx \log\left|\frac{\mu}{\sqrt{2}}\right| - \frac{\sigma^2}{2\mu^2 \ln[2]}.
% \end{equation}
% As $\frac{\sigma^2}{2\mu^2 \ln[2]} \rightarrow 0$ as $\mu/\sigma \rightarrow \infty$, we see that the convolution integral can be approximated for $\mu \gg \sigma$ as 
% \begin{align}
%     G_{\mathcal{N}(\mu,\sigma^2)}(\mu)=\int^{\infty}_{-\infty} \frac{\exp(-\frac{(x-\mu)^2}{2\sigma^2})}{\sigma \sqrt{2\pi}} \, \log \bigg[\frac{|x|}{\sqrt{2}} \bigg] dx \approx \log\left[\frac{|\mu|}{\sqrt{2}}\right].
% \end{align}
% as shown in Fig.~\ref{fig:fp_off_zero}, which shows that the value of the convolution integral is insensitive to the value of $\sigma$ when $\mu \gg \sigma$. 

% \noindent This means for a non-zero mean Gaussian random variable, for $\mu \gg \sigma$, $\Ht_s(\Xfp) \approx \Ht_s^\mu(X_{fp})$, with
% \begin{equation}
%     \label{eq:int_entropy}
%     \Ht^\mu_s(\Xfp) \triangleq \frac{1}{2}\log[2\pi e \sigma^2] + (p-1) - \log\bracket{|\mu| / \sqrt{2}}.
% \end{equation}


% \begin{lemma}[Bound on the Mercator Series Remainder]\label{lem:mercator-remainder}
% For all $|x| \le \frac{1}{2}$,
% \begin{equation}
%   \abs{\ln[1+x] - x + \frac{x^2}{2}} \leq \frac{2}{3}\,|x|^3.
% \end{equation}
% \end{lemma}
 
% \begin{proof}
% The Mercator series gives
% \begin{equation}
%   \ln\bracket{1+x} \;=\; \sum_{k=1}^{\infty} \frac{(-1)^{k+1}\, x^k}{k},
%   \qquad |x| < 1,
% \end{equation}
% so the second-order remainder is
% \begin{equation}
%   R_2(x)
%   \triangleq \ln\bracket{1+x} - x + \frac{x^2}{2}
%   \;=\; \sum_{k=3}^{\infty} \frac{(-1)^{k+1}\, x^k}{k}.
% \end{equation}
% By the triangle inequality and using the inequality $1/k \le 1/3$ for every $k \ge 3$,
% \begin{equation}
%   |R_2(x)|
%   \;\le\; \sum_{k=3}^{\infty} \frac{|x|^k}{k}
%   \;\le\; \frac{1}{3} \sum_{k=3}^{\infty} |x|^k
%   \;=\; \frac{1}{3} \cdot \frac{|x|^3}{1 - |x|},
% \end{equation}
% where the last equality is the geometric series
% $\sum_{k=3}^{\infty} |x|^k = |x|^3 \sum_{j=0}^{\infty} |x|^j = |x|^3/(1-|x|)$,
% valid for $|x| < 1$.
% Since $|x| \le \frac{1}{2}$ implies $1 - |x| \ge \frac{1}{2}$, we obtain
% \begin{equation}
%   |R_2(x)|
%   \;\le\; \frac{|x|^3}{3 \paren{\frac{1}{2}}}
%   \;=\; \frac{2}{3}\,|x|^3.
% \end{equation}
% \end{proof}

% \begin{lemma}\label{lem:Ac-bound}
% Let $\epsilon \sim N(0,\sigma^2)$, $\mu \neq 0$, and $A = \{|\epsilon/\mu| \le \frac{1}{2}\}$.
% Then,
% \begin{equation}
%   \E{\abs{\ln\abs{1+\frac{\epsilon}{\mu}}}\,\, \Bigr|\,A^c}P(A^c)
%   \leq \,\paren{\frac{C_1\sigma}{|\mu|} + \frac{C_2|\mu|}{\sigma}}\, e^{-|\mu|^2/8\sigma^2}
% \end{equation}
% for some $C_1, C_2 > 0$.
% In particular, the bound decays faster than any polynomial in~$|\mu|/\sigma$.
% \end{lemma}

% \begin{proof}
% Write $Z = \epsilon/\sigma \sim N(0,1)$, so that $\epsilon/\mu = \sigma Z/\mu$
% (taking $\mu>0$ without loss of generality; the case $\mu<0$ is symmetric).
% Set $\delta \triangleq 1 + \epsilon/\mu = 1 + \sigma Z/\mu$ and split
% \begin{equation}
%   A^c = A_1^c \cup A_2^c, \qquad
%   A_1^c \triangleq \left\{\abs{\frac{\epsilon}{\mu}}>\frac{1}{2}\right\} \cap \left\{\abs{\delta}\ge \frac{1}{2}\right\},\qquad
%   A_2^c \triangleq \left\{\abs{\frac{\epsilon}{\mu}}>\frac{1}{2}\right\} \cap \left\{\abs{\delta} < \frac{1}{2}\right\}.
% \end{equation}

% \medskip
% \noindent\textit{Contribution of~$A_1^c$.}\enspace
% For $t \ge \frac{1}{2}$ we have $|\ln t| \le \ln 2 + t$
% (since $-\ln t \leq \ln 2$ when $t \geq \frac{1}{2}$,
% and $\ln t \le t$ when $t > 0$).  Hence on~$A_1^c$,
% \begin{equation}
%   |\ln{\abs{\delta}}| \;\le\; \ln 2 + |\delta|
%   \;\le\; \ln 2 + 1 + |\frac{\epsilon}{\mu}|
% \end{equation}
% almost surely.
% Therefore
% \begin{align}
% &\abs{\ln|\delta|}\indic{A_1^c} \;\le\; \paren{\ln 2 + 1 + |\frac{\epsilon}{\mu}|}\indic{A_1^c}\\
%   \implies &\E{\abs{\ln\bracket{|\delta|}}\indic{A_1^c}}
%   \;\le\; \E{\paren{\ln 2 + 1 + |\frac{\epsilon}{\mu}|}\indic{A_1^c}}\\
%   \implies &\E{\abs{\ln\bracket{|\delta|}}\indic{A_1^c}}
%   \;\le\; (1+\ln 2)\,P(A_1^c) + \E{\abs{\frac{\sigma Z}{\mu}}\indic{A_1^c}}\\
%     \implies &\E{\abs{\ln\bracket{|\delta|}}\indic{A_1^c}}
%   \;\le\; (1+\ln 2)\,P(A^c) \;+\;
%     \frac{\sigma}{\mu}\E{|Z|\,\mathbf{1}_{|Z|>\mu/2\sigma}},
% \end{align}
% since $A_1^c \subset A^c \implies P(A_1^c) \leq P(A^c)$ and $\indic{A_1^c} \leq \indic{A^c}$ almost surely.
% From Eq.~\eqref{eq:p_ac_bound}, the Gaussian tail bound gives
% $P(A^c) \leq \frac{4\sigma}{\mu\sqrt{2\pi}}\,e^{-\mu^2/(8\sigma^2)}$,
% and the truncated first moment evaluates to
% \begin{equation}
%   \mathbb{E}\bigl[|Z|\,\mathbf{1}_{|Z|>a}\bigr]
%   = \frac{2}{\sqrt{2\pi}}\int_a^\infty ze^{-\frac{z^2}{2}}dz = \frac{2}{\sqrt{2\pi}}\,e^{-a^2/2},
%   \qquad a = \frac{\mu}{2\sigma}.
% \end{equation}
% Since \begin{equation}
%     \E{\abs{\ln\abs{\delta}} \,|\, A_1^c}P(A_1^c) = \E{\abs{\ln\abs{\delta}}\indic{A_1^c}} \leq \paren{\ln 2 + \frac{3}{2}}\frac{4\sigma}{\mu\sqrt{2\pi}}\,e^{-\mu^2/(8\sigma^2)},
% \end{equation}
% the entire $A_1^c$~contribution is at most
% $\frac{C_1\sigma}{\mu}\,e^{-\mu^2/(8\sigma^2)}$ for some constant~$C_1$.

% \medskip
% \noindent\textit{Contribution of~$A_2^c$.}\enspace
% On the event $\{|\delta|<\frac{1}{2}\}$ we have
% $\epsilon/\mu \in (-\frac{3}{2},-\frac{1}{2})$,
% i.e.\ $Z \in (-\frac{3\mu}{2\sigma},-\frac{\mu}{2\sigma})$.
% The density of~$\delta$ at a point~$t$ is
% $\frac{\mu}{\sigma}f_Z\paren{\frac{\mu}{\sigma}(t-1)}$,
% where $f_Z$ is the standard normal density.
% For $\abs{t}<\frac{1}{2}$ we have $(t-1)^2 \ge \frac{1}{4}$, giving the
% uniform density bound
% \begin{equation}
%   \frac{\mu}{\sigma}f_Z\paren{\frac{\mu}{\sigma}(t-1)}
%   = \frac{\mu}{\sigma\sqrt{2\pi}}e^{-\frac{\mu^2(t-1)^2}{2\sigma^2}}
%   \leq \frac{\mu}{\sigma\sqrt{2\pi}}\,e^{-\frac{\mu^2}{8\sigma^2}}.
% \end{equation}
% Since $\abs{\delta} < \frac{1}{2}$ almost surely implies $\abs{\frac{\epsilon}{\mu}}>\frac{1}{2}$ almost surely, we have $A_2^c = \{\abs{\delta} < \frac{1}{2}\}$ and
% \begin{equation}
%   \E{\abs{\ln\abs{\delta}}\,\indic{|\delta|<1/2}}
%   = \int_{-1/2}^{1/2}\frac{\mu}{\sigma}f_Z\paren{\frac{\mu}{\sigma}(t-1)}\abs{\ln\abs{t}}dt
%   \leq
%   \frac{\mu}{\sigma\sqrt{2\pi}}\,e^{-\frac{\mu^2}{8\sigma^2}}
%   \int_{-1/2}^{1/2} |\ln\abs{t}\,|\,dt.
% \end{equation}
% The integral evaluates to
% $-2\int_0^{1/2}\ln\bracket{t}\,dt = -2\bracket{t\ln t -t}\Bigr|_0^{1/2}
% = \ln 2 + 1$,
% so the $A_2^c$~contribution is at most
% $\frac{C_2\mu}{\sigma}\,e^{-\frac{\mu^2}{8\sigma^2}}$ for some constant $C_2$.

% \medskip
% \noindent\textit{Combining both contributions.}\enspace
% Adding both contributions yields
% \begin{equation}
%   \E{\abs{\ln\abs{1+\frac{\epsilon}{\mu}}}\,\mathbf{1}_{A^c}}
%   \;\le\; \paren{\frac{C_1\sigma}{\mu} + \frac{C_2\mu}{\sigma}} e^{-\frac{\mu^2}{8\sigma^2}}
% \end{equation}
% which decays faster than any polynomial in~$|\mu|/\sigma$.
% \end{proof}

% \textit{Approximating delta distribution: } Next, we can show the same result for a function which approximates a delta function as $\varepsilon \rightarrow 0$, provided $\mu \neq 0$. For a random variable $X$ where $f_X(x-\mu; \varepsilon) \rightarrow \delta (x-\mu)$ as $\varepsilon \rightarrow 0$ with $\mu \neq 0$, Eq.~\eqref{eq:G_int_non_gauss} becomes
% \begin{equation}
%     G_{f_X}(\mu) \triangleq \int^{\infty}_{-\infty} f_X(x-\mu; \epsilon) \log \bigg[\frac{|x|}{\sqrt{2}} \bigg] dx.
% \end{equation}
% As $\epsilon \rightarrow 0$, for any $\mu \neq 0$ such that $\log[|x| / \sqrt{2}]$ is continuous,
% \begin{align*}
%     G_{f_X}(\mu) & \approx \int^{\infty}_{-\infty} \delta(x-\mu) \log \bigg[\frac{|x|}{\sqrt{2}} \bigg] dx \\
%     & = \log \bigg[\frac{|\mu|}{\sqrt{2}} \bigg].
% \end{align*}
% Thus for any distribution, which may be non-Gaussian, if it approaches $\delta(\cdot)$ as a parameter $\epsilon$ which defines it approaches 0 and $\mu \neq 0$, in the limit of $\epsilon \rightarrow 0$ the integral term satisfies $G_{f_X}(\mu) \approx \log[|\mu|/\sqrt{2}]$, giving $\Ht_s(X_{fp}) \approx \Ht_s^\mu(X_{fp})$, where
% \begin{equation}
%     \Ht^\mu_s(\Xfp) \triangleq h(X) + (p-1) - \log\bracket{|\mu| / \sqrt{2}}.
% \end{equation}

% \FloatBarrier
\pagebreak
