# Supplementary material for: The Entropy of Floating-Point Numbers
Source: arXiv:2605.11546 source file (2026-09-02)
Supplement: Supplementary file 2 [file avg_sum_cost.tex]

\section{Landauer Cost of Averaging and Summing}\label{sec:avg_sum}
An even simpler prediction algorithm than linear regression is the average. Let the input to this algorithm be $X_1,\dots, X_n \iid f$, where $\E{X_i} = \mu$ and $\mathrm{var}\paren{X_i} = \sigma^2$. The differential entropy of the input is $h(X_1, \dots, X_n) = nh(X_1)$.

If $f$ is not Gaussian, for sufficiently large $n$, central limit theorem can be invoked to show that $\frac{1}{n}\sum\limits_{i = 1}^n X_i \Rightarrow \gauss{\mu}{\frac{\sigma^2}{n}}$ as $n \rightarrow \infty$. So the differential entropy of the final distribution is $h(\frac{1}{n}\sum\limits_{i = 1}^n X_i) \approx \frac{1}{2}\log\bracket{2\pi e \frac{\sigma^2}{n}}$. When $f_{X_i}$ is Gaussian, this is true even for small $n$.

For the case when $ \forall i, f_{X_i} \sim \gauss{0}{1}$ and the random variable are encoded in floating-point numbers with precision $p$, the discrete entropy difference is
\begin{align}
    \Delta H = n\Ht^0_{s}(p) - \Ht^0_{s}(p) = (n-1)\Ht^0_{s} \approx (n-1)(p + 2.46) \text{ bits,}\label{eq:landauer_avg}
\end{align}
where $\Ht^0_{s}(p)$ is derived in Section~\ref{sec:fpn}. Notice that Eq.~\eqref{eq:landauer_avg} is dominated by the number of inputs. As stressed in Section~\ref{sec:fpn}, $\Ht^0_{s}(p)$ does not depend on the variance of the random variable. This means that for zero-mean Gaussian random variables, the Landauer cost of averaging $\frac{1}{n}\sum\limits_{i = 1}^n X_i$ and summing $\sum\limits_{i = 1}^n X_i$ is equivalent, since $\sum\limits_{i = 1}^n X_i \sim \gauss{0}{n\sigma^2}$.




\FloatBarrier
\pagebreak
