# Supplementary material for: The Entropy of Floating-Point Numbers
Source: arXiv:2605.11546 source file (2026-09-02)
Supplement: Supplementary file 3 [file diff_entropy_z.tex]

\section{Computing the Differential Entropy of Z}\label{sec:compute_h_z}

\begin{lemma}\label{lem:diff_ent_Ex}
    Under the hypotheses of Lemma~\ref{lem:compute_f_z}, let $\psi(x) \triangleq \frac{d}{dx}\ln{\Gamma(x)} = \frac{\Gamma^\prime(x)}{\Gamma(x)}$ be the digamma function. The differential entropy of $Z$ is
\begin{align}
    \label{eq:diff_ent_Ex}
    h(Z) &= \log\bracket{e}\paren{\ln\bracket{\frac{\sigxi}{\sigx}} - \ln{\paren{\frac{\Gamma\paren{\frac{n+1}{2}}}{\sqrt{\pi}\Gamma\paren{\frac{n}{2}}}}} + \frac{n + 1}{2}\bracket{\psi\paren{\frac{n+1}{2}} - \psi\paren{\frac{n}{2}}}}.
\end{align}
\end{lemma}


\begin{proof}[Proof of Lemma~\ref{lem:diff_ent_Ex}]
    Using the distribution derived in Lemma~\ref{lem:compute_f_z}, the differential entropy of $Z$ is
\begin{align}
    &\frac{1}{\log\bracket{e}}h(Z) = -\int\limits_{-\infty}^\infty f_Z(z)\ln{f_Z(z)}dz\\
     &= -\int\limits_{-\infty}^\infty \paren{\sqrt{\frac{1}{\pi\paren{\sigx^2}^n\sigxi^2}}\frac{\Gamma\paren{\frac{n+1}{2}}}{\Gamma\paren{\frac{n}{2}}}\paren{\frac{\sigx^2\sigxi^2}{\sigx^2z^2 + \sigxi^2}}^{\frac{n + 1}{2}}}\\
     &\times\ln{\paren{\sqrt{\frac{1}{\pi\paren{\sigx^2}^n\sigxi^2}}\frac{\Gamma\paren{\frac{n+1}{2}}}{\Gamma\paren{\frac{n}{2}}}\paren{\frac{\sigx^2\sigxi^2}{\sigx^2z^2 + \sigxi^2}}^{\frac{n + 1}{2}}}}dz\\
     &= -\int\limits_{-\infty}^\infty \paren{\sqrt{\frac{1}{\pi\paren{\sigx^2}^n\sigxi^2}}\frac{\Gamma\paren{\frac{n+1}{2}}}{\Gamma\paren{\frac{n}{2}}}\paren{\frac{\sigx^2\sigxi^2}{\sigx^2z^2 + \sigxi^2}}^{\frac{n + 1}{2}}}\nonumber\\
     &\bracket{ \ln{\paren{\sqrt{\frac{1}{\pi\paren{\sigx^2}^n\sigxi^2}}\frac{\Gamma\paren{\frac{n+1}{2}}}{\Gamma\paren{\frac{n}{2}}}\paren{\sigxi^2}^{\frac{n + 1}{2}}}}- \frac{n + 1}{2}\ln\bracket{z^2 + \frac{\sigxi^2}{\sigx^2}}}dz\\
     &= -\sqrt{\frac{1}{\pi\paren{\sigx^2}^n\sigxi^2}}\frac{\Gamma\paren{\frac{n+1}{2}}}{\Gamma\paren{\frac{n}{2}}} \ln{\paren{\sqrt{\frac{1}{\pi\paren{\sigx^2}^n\sigxi^2}}\frac{\Gamma\paren{\frac{n+1}{2}}}{\Gamma\paren{\frac{n}{2}}}\paren{\sigxi^2}^{\frac{n + 1}{2}}}}\int\limits_{-\infty}^\infty \paren{\frac{\sigx^2\sigxi^2}{\sigx^2z^2 + \sigxi^2}}^{\frac{n + 1}{2}} dz\\
     &+ \frac{n + 1}{2}\sqrt{\frac{1}{\pi\paren{\sigx^2}^n\sigxi^2}}\frac{\Gamma\paren{\frac{n+1}{2}}}{\Gamma\paren{\frac{n}{2}}}\int\limits_{-\infty}^\infty \paren{\frac{\sigx^2\sigxi^2}{\sigx^2z^2 + \sigxi^2}}^{\frac{n + 1}{2}}\ln\bracket{z^2 + \frac{\sigxi^2}{\sigx^2}}dz\\
     &= - \ln{\paren{\sqrt{\frac{1}{\pi\paren{\sigx^2}^n\sigxi^2}}\frac{\Gamma\paren{\frac{n+1}{2}}}{\Gamma\paren{\frac{n}{2}}}\paren{\sigxi^2}^{\frac{n + 1}{2}}}}\nonumber\\
     &+ \frac{n + 1}{2}\sqrt{\frac{1}{\pi\paren{\sigx^2}^n\sigxi^2}}\frac{\Gamma\paren{\frac{n+1}{2}}}{\Gamma\paren{\frac{n}{2}}}\int\limits_{-\infty}^\infty \paren{\frac{\sigx^2\sigxi^2}{\sigx^2z^2 + \sigxi^2}}^{\frac{n + 1}{2}}\ln\bracket{z^2 + \frac{\sigxi^2}{\sigx^2}}dz\label{eq:normalized}
\end{align}

The first term in Eq.~\eqref{eq:normalized} is due to $f_Z(z)$ being a probability density function.

Just solving for $\int\limits_{-\infty}^\infty \paren{\frac{\sigx^2\sigxi^2}{\sigx^2z^2 + \sigxi^2}}^{\frac{n + 1}{2}}\ln\bracket{z^2 + \frac{\sigxi^2}{\sigx^2}}dz$, let $\psi(x) \triangleq \frac{d}{dx}\ln{\Gamma(x)} = \frac{\Gamma^\prime(x)}{\Gamma(x)}$. Using the change of variables $\theta = \tan^{-1}(\frac{\sigx z}{\sigxi})$,


\begin{align}
    &\int\limits_{-\infty}^\infty \paren{\frac{\sigx^2\sigxi^2}{\sigx^2z^2 + \sigxi^2}}^{\frac{n + 1}{2}}\ln\bracket{z^2 + \frac{\sigxi^2}{\sigx^2}}dz = \sigx^n\sigxi\int\limits_{-\frac{\pi}{2}}^\frac{\pi}{2} \paren{\frac{1}{\sec^2{\theta}}}^{\frac{n - 1}{2}}\ln\bracket{\frac{\sigxi^2}{\sigx^2}\sec^2\theta}d\theta\\
    &=  \sigx^n\sigxi\bracket{\int\limits_{-\frac{\pi}{2}}^\frac{\pi}{2} \paren{\frac{1}{\sec^2{\theta}}}^{\frac{n-1}{2}}\ln\bracket{\sec^2\theta}d\theta + \ln\bracket{\frac{\sigxi^2}{\sigx^2}}\int\limits_{-\frac{\pi}{2}}^\frac{\pi}{2} \paren{\frac{1}{\sec^2{\theta}}}^{\frac{n-1}{2}}d\theta}\\
    &=  \sigx^n\sigxi\bracket{\frac{\sqrt{\pi}\Gamma\paren{\frac{n}{2}}\paren{\psi\paren{\frac{n+1}{2}} - \psi\paren{\frac{n}{2}}}}{\Gamma\paren{\frac{n+1}{2}}}  + \frac{\ln\bracket{\frac{\sigxi^2}{\sigx^2}}\sqrt{\pi}\Gamma\paren{\frac{n}{2}}  }{\Gamma\paren{\frac{n+1}{2}}}}\\
    &= \frac{ \sigx^n\sigxi\sqrt{\pi}\Gamma\paren{\frac{n}{2}}}{\Gamma\paren{\frac{n+1}{2}}}\bracket{\psi\paren{\frac{n+1}{2}} - \psi\paren{\frac{n}{2}} + \ln\bracket{\frac{\sigxi^2}{\sigx^2}}}.
\end{align}

Now returning to the computation of $h(Z)$, we have
\begin{align}
    \frac{1}{\log\bracket{e}}h(Z) &= - \ln{\paren{\sqrt{\frac{1}{\pi\paren{\sigx^2}^n\sigxi^2}}\frac{\Gamma\paren{\frac{n+1}{2}}}{\Gamma\paren{\frac{n}{2}}}\paren{\sigxi^2}^{\frac{n + 1}{2}}}}\nonumber\\ 
    &+ \frac{n + 1}{2}\bracket{\psi\paren{\frac{n+1}{2}} - \psi\paren{\frac{n}{2}} + \ln\bracket{\frac{\sigxi^2}{\sigx^2}}}\\
    &= - \ln{\paren{\frac{\sigxi^n}{\sqrt{\pi}\sigx^n}\frac{\Gamma\paren{\frac{n+1}{2}}}{\Gamma\paren{\frac{n}{2}}}}} + \frac{n + 1}{2}\bracket{\psi\paren{\frac{n+1}{2}} - \psi\paren{\frac{n}{2}} + \ln\bracket{\frac{\sigxi^2}{\sigx^2}}}\\
    &= \ln\bracket{\frac{\sigxi}{\sigx}} - \ln{\paren{\frac{\Gamma\paren{\frac{n+1}{2}}}{\sqrt{\pi}\Gamma\paren{\frac{n}{2}}}}} + \frac{n + 1}{2}\bracket{\psi\paren{\frac{n+1}{2}} - \psi\paren{\frac{n}{2}}}.
\end{align}
\end{proof}

\begin{figure}[htbp]
  \centering
  \begin{subfigure}{0.4\textwidth}
    \centering
    \includegraphics[width=\linewidth]{code/quantized_entropy_midpoint/exact_lr/H_wh_fp_vs_n.pdf}
    \caption{}
    \label{fig:H_fp_wh_exact}
  \end{subfigure}
  \begin{subfigure}{0.4\textwidth}
    \centering
    \includegraphics[width=\linewidth]{code/quantized_entropy_midpoint/exact_lr/landauer_cost_per_n_vs_n.pdf}
    \caption{}
    \label{fig:Ex_dH_exact}
  \end{subfigure}\hfill
  \caption{\textit{The Landauer cost for exact zero-intercept simple linear regression.} Input and output states are floating-point numbers with $p = 4$ and $E=4$. The candidate values of the $SNR = \frac{w^2\sigx^2}{\sigxi^2}$ are $0.062$, $0.25$, $1$, $4$, and $25$. (\ref{fig:H_fp_wh_exact}) The output model entropy, and its dependence on the data size $n$ and ground truth $w$. (\ref{fig:Ex_dH_exact}) The entropy difference for various values of SNR and a range of $n$.}
  \label{fig:exact_lr_ent}
\end{figure}



\FloatBarrier
\pagebreak
