# Supplementary material for: The Entropy of Floating-Point Numbers
Source: arXiv:2605.11546 source file (2026-09-02)
Supplement: Supplementary file 4 [file extended_kostina_proofs.tex]

\section{Extending Theorem's in Kostina Paper to Float Setting}

\thinkabout{Midpoint quantization is dealing with L1 norm nearest neighbors instead of L2 norm. Noting that this product lattice structure, where each coordinate is quantized independently, is inefficient (check \cite[section 4.e]{GrayNeuhoff1998Quantization}). In 1D, all of the $L^p$ norms are just the absolute value.}

\begin{theorem}[Kostina, Theorem 8, bound on $\relent{X}{X_\mathcal{C}}$. Particularized to scalar case, and extended to nonuniform bins]
Let $X$ be a random variable with $h(X) > -\infty$ and $v$-regular density. Let $q: \R{} \mapsto \R{}$ be a quantizer with cells $\{\mathcal{V}_c\}$. Then the information random variable and the entropy at the output of the lattice quantizer can be bounded as
\begin{align}
\imath(q_{\mathcal{C}}(x)) &\leq \log \frac{1}{f_X(x)} - \log \Delta(x) + \Delta(x) v_{\mathcal{C}}(x) \log e, \label{eq:info_bound} \\
H(q_{\mathcal{C}}(X)) &\leq h(X) - \E{\log \Delta(X)} + \E{\Delta(X)v_{\mathcal{C}}(X)} \log e, \label{eq:entropy_bound}
\end{align}
where for each representable value $c$, $r_{c} = \max\limits_{x \in \mathcal{V}_{c}}\norm{x - c}{2}$ is the lattice covering radius, and $v_{\mathcal{C}}(x)$ is given by
\begin{equation}
v_{\mathcal{C}}(x) = \max_{u \in \mathcal{V}_{\mathcal{C}}(q_{\mathcal{C}}(x))} v(u).
\end{equation}
% Furthermore, if $v(x) = v(\norm{x}{2})$ is convex and nondecreasing, then \eqref{eq:info_bound} and \eqref{eq:entropy_bound} can be strengthened by replacing the above with
% \begin{equation}
% v_{\mathcal{C}}(x) = \frac{1}{2} v(\norm{x}{2}) + \frac{1}{2} v(\norm{x}{2} + 2r_{\mathcal{C}}),
% \end{equation}
% and if $v(x) = c_1 \norm{x}{2} + c_0$, then this particularizes as
% \begin{equation}
% v_{\mathcal{C}}(x) = c_1 \norm{x}{2} + c_1 r_{\mathcal{C}} + c_0.
% \end{equation}
\end{theorem}

\begin{proof}
Observe that,
\begin{align}
|\log f_X(a) - \log f_X(b)|
&= \left| \int_0^1 \innprod{\nabla \log f_X(ta + (1-t)b)}{a - b} \, dt \right| \\
&\leq \norm{a - b}{2} \log e \int_0^1 v(ta + (1-t)b) \, dt\label{eq:cauchyschwarz} \\
&\leq \max_{0 \leq t \leq 1} v(ta + (1-t)b) \norm{a - b}{2} \log e,\label{eq:logbound}
\end{align}
where \eqref{eq:cauchyschwarz} holds by Cauchy-Schwarz inequality. 
\thinkabout{Since $\norm{x}{2}\leq \norm{x}{1}$ we could have a looser bound wrt the $\norm{\cdot}{1}$ norm.}

For each $c \in \mathcal{C}$, $f_{X_c}(c - u_c) = \frac{P\{X \in \mathcal{V}_\mathcal{C}(c)\}}{\Delta(c)}$. Let $U_c \sim \unif{- \frac{\Delta(c)}{2}}{\frac{\Delta(c)}{2}}$, for all $u \in [- \frac{\Delta(c)}{2}, \frac{\Delta(c)}{2}]$, we have 
\begin{align}
    f_{X_c}(c - u) = \E{f_X(c + U_c)},
\end{align}
so by the MVT, there exists a $u_c \in  [- \frac{\Delta(c)}{2}, \frac{\Delta(c)}{2}]$ where
\begin{equation}
f_X(c - u_c) = f_{X_c}(c - u).\label{eq:mvt}
\end{equation}


Using \eqref{eq:mvt} and \eqref{eq:logbound} with $a=x$ and $b =q_{\mathcal{C}}(x) - u_c$, we evaluate the information in $q_{\mathcal{C}}(x)$ as
\begin{align}
\imath(q_{\mathcal{C}}(x))
&= \log \frac{1}{f_{X_{\mathcal{C}}}(x)} - \log \Delta(x) \\
&= \log \frac{1}{f_X(x)} - \log \Delta(x) + \log \frac{f_X(x)}{f_X(q_{\mathcal{C}}(x) - u_c)} \\
&\leq \log \frac{1}{f_X(x)} - \log \Delta(x)\nonumber\\ & + \max_{0 \leq t \leq 1} v(tx + (1-t)(q_{\mathcal{C}}(x) - u_c)) \norm{x - \paren{q_{\mathcal{C}}(x) - u_c}}{2} \log e\label{eq:preconvexity}\\
&\leq \log \frac{1}{f_X(x)} - \log \Delta(x)\nonumber\\ & + v_{\mathcal{C}}(x)\paren{\norm{x - q_{\mathcal{C}}(x)}{2} + \norm{u_c}{2}} \log e\label{eq:convexityrequired}\\
&\leq \log \frac{1}{f_X(x)} - \log \Delta(x) + \Delta(x)v_{\mathcal{C}}(x) \log e\\
&= \log \frac{1}{f_X(x)} - \log \Delta(x)+ 2r_{c}(x) v_{\mathcal{C}}(x) \log e,
\end{align}
which is equivalent to \eqref{eq:info_bound}, and \eqref{eq:entropy_bound} is immediate upon taking an expectation of \eqref{eq:info_bound}.



\thinkabout{There are nuances that come with higher dimension. In the above proof, going from \eqref{eq:preconvexity} to \eqref{eq:convexityrequired} requires convexity of each cell, and this might not hold for midpoint quantization due to the L1 nearest neighbors as opposed to L2. Need to check if the proof will still go through. Convexity of each cell hold trivially for the scalar case. For the scalar case $r_\mathcal{C} = \Delta/2$, but for a cubic lattice in $\R{n}$, $r_\mathcal{C} = 1/2\sqrt{\sum_{i = 1}^{n}\Delta^2} = \frac{\sqrt{n}\Delta}{2}$. A spherical lattice has a different scaling. $\rho_\mathcal{C}$ in the Kostina paper quantifies these different scalings.}



% If $v(x) = v(\norm{x}{2})$, convex and nondecreasing, we strengthen (128) by applying Jensen's inequality to (127):
% \begin{align}
% |\log f_X(a) - \log f_X(b)|
% &\leq \frac{\log e}{2} (v(\norm{a}{2}) + v(\norm{b}{2})) \norm{a - b}{2} \\
% &\leq \log e (v(\norm{a}{2}) + v(\norm{a}{2} + 2r_{\mathcal{C}})) r_{\mathcal{C}},
% \end{align}
% where to get (133) we used the triangle inequality, the assumption that $v$ is nondecreasing, and the fact that $\norm{a - b}{2} \leq 2r_{\mathcal{C}}$ for $a$ and $b$ from the same quantization cell. Modifying (131) accordingly results in a strengthening of (121) and (122) with $v_{\mathcal{C}}$ in (124).
\end{proof}
