# Supplementary material for: The Entropy of Floating-Point Numbers
Source: arXiv:2605.11546 source file (2026-09-02)
Supplement: Supplementary file 5 [file gaussian_approx.tex]

\section{Applying approximations to the Gaussian case}\label{app:FPN_app_gauss}

Here the theorems for the floating point entropy of Gaussian random variables are reviewed. See Figure~\ref{fig:fp_exponents} for a directly computed histogram of exponent values. Directly computing the entropy of the histograms returns a discrete entropy of $\sim 2.54$ bits, which is close to the offset factor above the mantissa contribution $p$ in $\Ht^0_s(p) \approx p + 2.46$ bits. Since bin sizes are fairly large with respect to the underlying distribution of exponents, this divergence likely can be explained by quantization noise.

\begin{figure}[htbp]
  \centering
    \includegraphics[width=0.36\linewidth]{fpn/exponents (2).pdf}
\caption{\textit{Histogram of exponent values for a normally distributed random variable.} The distribution of exponent states for $X \sim \mathcal{N}(0,\sigma^2)$. From left to right, the distributions plotted have $\sigma = \{10^{-3}, 10^0, 10^3 \}$. All three have a discrete entropy $H(\log[X]) \approx 2.54$ bits. These distributions conform well to observational data in \cite{bordawekar2022efloatentropycodedfloatingpoint, hao_neuzip_2024}.}
    \label{fig:fp_exponents}
\end{figure}

\begin{theorem}[Approximating the entropy of a mean-zero univariate gaussian]
    \label{thm:single_gaussian}
    The discrete entropy of a zero-mean normally distributed continuous random variable $X \sim \mathcal{N}(0, \sigma_x^2)$ as represented on a floating-point number, with the approximations specified by Eq.~\eqref{eq:diff_approx} and~\eqref{eq:step_approx} applied, is a constant specified by the floating point number's precision, $p$.
    \begin{equation}
        \tilde H_s(X_{fp}) = (p-1) + \frac{1}{2} \log[2 \pi e] + 1 + \frac{\gamma_e}{2\ln[2]}
    \end{equation}
    
\end{theorem}
\begin{proof}
    Let $X \sim \mathcal{N}(0, \sigma_x^2)$.
    \begin{equation}
    \begin{aligned}
    \label{eq:1d-0m-fp}
        \Ht_{s}(\Xfp) &\triangleq h(X) - \E{\log[\Delta_s(x)]} \\
        &= \frac{1}{2}\log[2\pi e \sigma^2_x] - \int^{\infty}_{-\infty} \frac{\exp(-\frac{x^2}{2\sigma_x^2})}{\sigma_x \sqrt{2\pi}} \log [\Delta_s(x)] \, dx  \\
        &= \frac{1}{2}\log[2\pi e \sigma^2_x] - \int^{\infty}_{-\infty} \frac{\exp(-\frac{x^2}{2\sigma_x^2})}{\sigma_x \sqrt{2\pi}} (\log[|x|/\sqrt{2}] - (p - 1)) \, dx \\
        & = \frac{1}{2}\log[2\pi e \sigma^2_x] + (p - 1) - 2\int^{\infty}_0 \frac{\exp(-\frac{x^2}{2\sigma_x^2})}{\sigma_x \sqrt{2\pi}} \log[x/\sqrt{2}] \, dx\\
        & = \frac{1}{2}\log[2\pi e \sigma^2_x] + (p-1) + \bigg(1 + \frac{\gamma_e}{2\ln[2]} -\frac{1}{2} \log[\sigma^2_x] \bigg)\\
        & = (p-1) + \frac{1}{2} \log[2 \pi e] + 1 + \frac{\gamma_e}{2\ln[2]}\\
        & = p + \frac{1}{2} \log[2 \pi e] + \frac{\gamma_e}{2\ln[2]}.
    \end{aligned}
\end{equation}
\end{proof}

\begin{theorem}
    \label{thm:double_gaussian}
    Let $X \sim \mathcal{N}(0,\sigma_x^2)$, $\Xi \sim \mathcal{N}(0,\sigma_\xi^2)$, $w \in \mathbb{R}$, and $Y = wX + \Xi$. The approximate joint discrete entropy of $(\Xfp, \Yfp)$ is,
\begin{equation*}
    \Ht_s(\Xfp, \Yfp) = 2 \Ht^0_s(p)-\frac{1}{2} \log \bigg [ 1+\frac{\sigma_x^2 w^2}{\sigma_\xi^2} \bigg].
\end{equation*}
\end{theorem}
\begin{proof}
\begin{equation}
\label{eq:approx_joint_ent_SNR_start}
    \begin{aligned}
        \Ht_s(\Xfp, \Yfp) &\triangleq h(X, Y) - \iint_{-\infty}^\infty f_{XY}(x,y) ( \log[\Delta_s(x)] + \log[\Delta_s(y)])dxdy \\
        = h& (X)  + h(\Xi) - \iint_{-\infty}^\infty f_{XY}(x,y)  \log[\Delta_s(x)] dxdy - \iint_{-\infty}^\infty f_{XY}(x,y)\log[\Delta_s(y)]dxdy \\
        = \frac{1}{2}&\log[2\pi e \sigma_x^2] + \frac{1}{2}\log[2\pi e \sigma_\xi^2] - \int_{-\infty}^\infty f_{X}(x)  \log[\Delta_s(x)] dx - \int_{-\infty}^\infty f_{Y}(y)\log[\Delta_s(y)]dy.
    \end{aligned}
\end{equation}
where $h(X,Y) = h(X) + h(\Xi)$ is because $X$ is independent from $\Xi$ and $(X,\Xi) \mapsto (X,Y)$ is an invertible linear transformation with Jacobian 1. The expressions follow directly from the differential entropy of a normal distribution \cite{CoverThomas}. In the last line, $f_X(x)$ and $f_Y(y)$ are the marginal distributions over $f_{XY}(x,y)$,
\begin{equation}
    f_X(x) = \int_{-\infty}^\infty f_{XY}(x,y) \, dy\text{,  }f_Y(y) = \int_{-\infty}^\infty f_{XY}(x,y) \, dx,
\end{equation}
where from Eq.~\eqref{eq:initial_dist}
\begin{equation}
    f_X(x) =
\frac{1}{\sqrt{2\pi\sigma_x^2}}
\exp\left(-\frac{x^2}{2\sigma_x^2}\right)\text{,  } f_Y(y) =
\frac{1}{\sqrt{2\pi(\sigma_\xi^2+w^2\sigma_x^2)}}
\exp\left(-\frac{y^2}{2(\sigma_\xi^2+w^2\sigma_x^2)}\right).
\end{equation}
Applying the same steps as in Theorem~\ref{thm:single_gaussian} to evaluate the bin terms, we obtain
\begin{equation}
    \int_{-\infty}^{\infty} f_X(x)\,\log\bracket{\Delta_s(x)}\,dx
\approx
-\left(p+\frac{\gamma_e}{2\ln 2}\right)
+\frac{1}{2}\log \sigma_x^2,
\end{equation}

\begin{equation}
    \int_{-\infty}^{\infty} f_Y(y)\,\log\bracket{\Delta_s (y)}\,dy
    \approx
    -\left(p+\frac{\gamma_e}{2\ln 2}\right)
    +\frac{1}{2}\log\bracket{\sigma_\xi^2+w^2\sigma_x^2}.
\end{equation}
Plugging these back into the original expression, we obtain
\begin{equation}
    \label{eq:approx_joint_ent_SNR_app}
    \begin{aligned}
        \Ht_s(\Xfp, \Yfp) &= \frac{1}{2}\log[2\pi e \sigma_x^2] + \frac{1}{2}\log[2\pi e \sigma_\xi^2] + p+\frac{\gamma_e}{2\ln 2} - \frac{1}{2}\log \sigma_x^2\\
        & + p + \frac{\gamma_e}{2\ln[2]} - \frac{1}{2} \log[\sigma^2_\xi + \sigma_x^2 w^2].
    \end{aligned}
\end{equation}
Using the definition $H^0_s(p)$ from definition Eq.~\eqref{eq:single_mean_0} and Theorem~\ref{thm:single_gaussian}, we can obtain a clean final expression,
\begin{equation}
    \Ht_s(\Xfp, \Yfp) = 2 \Ht^0_s(p)-\frac{1}{2} \log \bigg [ 1+\frac{\sigma_x^2 w^2}{\sigma_\xi^2} \bigg]
\end{equation}
\end{proof}
