# Supplementary material for: The Entropy of Floating-Point Numbers
Source: arXiv:2605.11546 source file (2026-09-02)
Supplement: Supplementary file 6 [file mismatch_cost_app.tex]

\section{Mismatch Cost}
\label{app:mmc}

\subsubsection{Defining $\Delta S_{env}$ and $\Delta S_{tot}$ with a Continuous Time Markov Chain}

One general way to model such a time dependence is via a continuous time Markov chain (CTMC) based on transition rates between states of the joint computational system \cite{Wolpert2019, Manzano2024, KolchinskyWolpert2021, Owen_2019, esposito2010}. In this case, the dynamics of the computational system are fixed by a time varying matrix $W_{x_c,x_c'}(t)$, which defines the rate of transitions between states $x_c, x_c'\in \mathcal{X}_c$ at time $t$ \cite{Wolpert2019, KolchinskyWolpert2021}. 
While running an algorithm, the computational system evolves according to
\begin{equation}
    \label{eq:CTMC}
    \frac{d}{dt} p(x_c,t) = \sum_{x'_c \in \mathcal{X}_c} W_{x_c;x_c'}(t) p(x_c',t).
\end{equation}
For these dynamics, \cite{esposito2010} shows
\begin{equation}
    \Delta S_{sys} = -k_B \ln[2] \int^{t_f}_0 \sum_{x_c,x_c' \in \mathcal{X}_c} W_{x_c,x_c'}(t)p(x_c', t) \log \bigg[ \frac{p(x_c,t)}{p(x_c',t)} \bigg]dt,
\end{equation}
\begin{equation}
    \label{eq:s_env}
    \Delta S_{env} = - k_B \ln[2] \int^{t_f}_0\sum_{x_c,x_c'\in \mathcal{X}_c} W_{x_c,x_c'}(t) p(x_c', t) \log \bigg[ \frac{W_{x_c',x_c}(t)}{W_{x_c,x_c'}(t)} \bigg] dt,
\end{equation}
\begin{equation}
    \Delta S_{tot} = k_B \ln[2] \int^{t_f}_0\sum_{x_c,x_c'\in \mathcal{X}_c} W_{x_c,x_c'}(t) p(x_c', t) \log \bigg[ \frac{W_{x_c,x_c'}(t)p(x_c',t)}{W_{x_c',x_c}(t) p(x_c,t)} \bigg] dt.
\end{equation}
If the transition rates $W_{x_c,x_c'}$ satisfy $\ln[W_{x_c,x_c'}/W_{x_c',x_c}] = (E(x_c') - E(x_c))/(k_BT)$, where $E(x_c)$ is an energy function over computational states, then we can say the average heat is given by $Q = T \Delta S_{env}$ \cite[p.30]{Wolpert2019} \cite{Seifert_2012}. This implies that the average heat output, fixed by Eqs.~\eqref{eq:CTMC},~\eqref{eq:s_env} is given by $Q = T(-\Delta S_{sys} + \Delta S_{tot}) = \Delta E_{min} +T\Delta S_{tot}$. 












Let $\compsimplex$ denote the probability simplex associated with the computational state space $\mathcal{X}_c$. We can think of the computation which takes us from $p_1 \in \compsimplex$ to $p_{F-1} \in \compsimplex$ as fixed by a conditional distribution $\pi(x_c|x_c')$, which determines $p_{F-1}$ from $p_1$ by
\begin{equation}
    p_{F-1}(x_c) = \sum_{x_c'\in \mathcal{X}_c} \pi(x_c|x_c') p_1(x_c').
\end{equation}
The conditional distribution $\pi(x_c|x_c')$ can be physically implemented to infinitesimally small error by the time-protocol of the rate matrix $W_{x_c,x_c'}(t)$ \cite[p. 23]{Wolpert2019}\cite{Owen_2019} (assuming $x_c$ [or $x_M$] is extended to include sufficient states, see \cite{Owen_2019}). The notation $p_{F-1} = \pi p_1$ emphasizes that $p_{F-1}$ is purely a function of the input state $p_1$ and the physical manipulations performed by the computation $W_{x_c,x_c'}(t)$, which determines $\pi(x_c|x_c')$.

\subsubsection{Variational MMC and the Island Decomposition}

The requirements to obtain the minimum entropy distribution $q_1$ that returns a unique MMC are specified in \cite{Wolpert_2020}. \cite{Wolpert_2020} points out that uniqueness of optimal distributions can only be verified for `islands' of the conditional distribution defined by the algorithm. 
We can describe an algorithm (possibly stochastic) as implementing a conditional distribution $\pi(x_c | x_c')$ that maps between computational states $x_c,x_c' \in \mathcal{X}_c$. The islands of the algorithm are specified by the following relation for $x_c, x'_c \in \mathcal{X}_c$:
\begin{equation}
    \label{eq:Islands}
    x_c \sim x_c' \Leftrightarrow \exists x_f \in \mathcal{X}_c : \pi(x_f|x_c') > 0, \pi(x_f|x_c) > 0,
\end{equation}
meaning there is a finite probability of $x_c$ and $x_c'$ transitioning to the same state $x_f$. An \textit{island} of $\pi(x_c | x_c')$ is a connected subset of $\mathcal{X}_c$ given by the transitive closure of Eq.~\eqref{eq:Islands}. The set of islands of $\pi$ partition $\mathcal{X}_c$, where the set of islands is denoted $L(\pi)$.

We can consider the distribution over an island $c \in L(\pi)$, given by $p^c(x_c) = \indic{x_c \in c}p(x_c)/p(c)$. If optimized over a the probability simplex specific to the island $c$ is $\boldsymbol{\Delta}_c$, the minimizer $q^c(x)$ will be unique \cite{Wolpert_2020}. The total distribution optimized over $\compsimplex$ can be decomposed in terms of islands and the probability of their individual occupation $q_1(c)$, 
\begin{equation}
    \label{eq:island_dist}
    q_1(x_c) = \sum_{c \in L(\pi)} q_1(c) q_1^c(x_c).
\end{equation}
The factors $q(c)$ do not contribute to the KL divergences in Eq.~\eqref{eq:MMC}, meaning they do not contribute to the MMC and ensuring the MMC is unique for the optimal distribution $q_1$.

For a deterministic algorithm, $\pi$ will be valued 0 or 1 for all inputs. In this case, the islands of the algorithm will be specified by the set of inputs that correspond to a single output state. As we have considered them, both exact linear regression and SGD are deterministic algorithms. In the exact case, the final $\wh_Q$ follows deterministically from the data $\mathcal{D}_Q$, and given that for SGD $\wh_Q$ has a deterministic initialization, the final $\wh_Q$ also follows deterministically from the batches $\{\mathcal{B}_{Q,1},...,\mathcal{B}_{Q,\tau}\}$. Each island of the algorithms corresponds to all possible $\mathcal{D}_Q$ or $\{\mathcal{B}_{Q,1},...,\mathcal{B}_{Q,\tau}\}$ that have the same output $\wh_Q$. For both the exact regression and SGD, the islands of input states are complex but disjoint subsets of the input data, which correspond to specific values of $\Wh$, rendering the island decomposition difficult to consider in this case.

The variational approach breaks the island decomposition by preventing $q_1^c(x_c)$ from being individually optimized, and by preventing a description of the input state as specified by Eq.~\eqref{eq:island_dist}. With a variational $q_{1,v}$ that breaks the island decomposition, we cannot guarantee it to be unique. However, this lack of uniqueness does not prevent MMC$_v$ from providing a lower bound on the true MMC: one can perform a bounded optimization to find $q_{1,v}$, which may or may not be unique, the difference MMC$_v = \Delta S_{tot}(p_{1,v}) - \Delta S_{tot}(q_{1,v})$ will retain the property $0 \leq $ MMC$_v \leq $ MMC for variational distributions $p_{1,v} \in \mathcal{V}$. 

\subsubsection{Illustrative MMC for exact regression and SGD}

\FloatBarrier
\begin{figure}[htbp]
    \centering
    \begin{subfigure}{0.36\textwidth}
        \includegraphics[width=\linewidth]{MMC/MMC_Ex.pdf}
        \caption{}
        \label{fig:MMC_Ex}
    \end{subfigure}
    \begin{subfigure}{0.42\textwidth}
        \includegraphics[width=\linewidth]{MMC/MMC_SGD.pdf}
        \caption{}
        \label{fig:MMC_SGD}
    \end{subfigure}
    \caption{\textit{A lower bound on the mismatch cost for continuously parameterized inputs}. MMC$_v(\sigma_x, \sigma_\xi)$ as a function of $\sigma_x$ and $\sigma_\xi$, with each plot assumes the entropy flow $\Delta S_{env,Ex} = \Delta S_{env, SGD} = C + \alpha(\sigma_x^2 + \sigma_\xi^2 )$, and $w = 1$. A bounded optimization is performed for for $0.75 \leq \sigma_x \leq 5$, $0.5 \leq \sigma_\xi \leq 5$. \ref{fig:MMC_Ex} A sample MMC$_v$ landscape for exact linear regression with the illustrative $\Delta S_{env,Ex}=C + \alpha(\sigma_x^2 + \sigma_\xi^2 )$, and $n = 10$. \ref{fig:MMC_SGD} A sample MMC$_v$ landscape for linear regression via SGD with an illustrative $\Delta S_{env,SGD}=C + \alpha(\sigma_x^2 + \sigma_\xi^2 )$, and $B = 1$, $\tau = 50$.} 
    \label{fig:MMC}
\end{figure}

For exact regression, the variational family will be $\theta = (\sigma_x,\sigma_\xi)$, which only runs from inputs to outputs once, $\Delta S_{tot}$ will be
\begin{equation}
    \Delta S_{tot, Ex}(\sigma_x, \sigma_\xi) = -E^{Ex}_{min}(\sigma_x,\sigma_\xi)/T+\Delta S_{env,Ex}(\sigma_x,\sigma_\xi)
\end{equation}
from which $q_{1,v}(\sigma_x^\star,\sigma_\xi^\star)$, defined by the optimal $\sigma_x^\star$ and $\sigma_\xi^\star$, follows from Eq.~\eqref{eq:mmc_var_opt}. MMC$_v$ for exact regression is given by MMC$_v(\sigma_x,\sigma_\xi) = \Delta S_{tot, Ex}(\sigma_x,\sigma_\xi) - \Delta S_{tot,Ex}(\sigma_x^\star,\sigma_\xi^\star)$. Fixing $\Delta S_{env,Ex} = C+\alpha(\sigma_x^2 + \sigma_\xi^2)$, MMC$_v$ is plotted for a range of distributions in Fig.~\ref{fig:MMC_Ex}.

For the SGD device, each update cycle $k$ takes input $(\mathcal{B}_Q, \hat{W}_{Q,k})$ and produces
output $\hat{W}_{Q,k+1}$, constituting a separate physical process. The MMC should
therefore be evaluated at each step and summed,
\begin{equation}
    \mathrm{MMC}_{v,\mathrm{SGD}}(\sigma_x,\sigma_\xi) = \sum_{k=0}^{\tau-1} \Bigl(\Delta S_{tot, k}(\sigma_x,\sigma_\xi) - \Delta S_{tot,k}(\sigma_x^\star,\sigma_\xi^\star)\Bigr),
\end{equation}
where the per-step total entropy production is
\begin{equation}
    \Delta S_{\mathrm{tot},k}(\sigma_x, \sigma_\xi)
    = 
    - k_B \ln[2]\left(H(\hat{W}_{Q,k}) + B H(X_{fp}, Y_{fp})
      - H(\hat{W}_{Q,k+1})\right) + \Delta S_{env,SGD}.
\end{equation}
To simplify this expression, we can assume that the entropy flow at each step depends only
on the batch distribution, and not on the evolving model parameter distribution,
\begin{equation}
    \Delta S_{env,k}(\theta) = \Delta S_{env,Ex}(\theta)/\tau =  (C + \alpha(\sigma_x^2 + \sigma_\xi^2))/\tau \quad \forall\, k.
\end{equation}
This reduces the per-step sum to a telescoping series as in the preliminaries, giving the total entropy production
\begin{equation}
    \Delta S_{tot,\mathrm{SGD}}(\sigma_x,\sigma_\xi) = -E^{SGD}_{min}(\sigma_x,\sigma_\xi)/T + \Delta S_{env,SGD}(\sigma_x,\sigma_\xi),
\end{equation}
and thus $\mathrm{MMC}_{v,\mathrm{SGD}}(\sigma_x,\sigma_\xi) = \Delta S_{tot,\mathrm{SGD}}(\sigma_x,\sigma_\xi) - \Delta S_{tot,\mathrm{SGD}}(\sigma_x^\star,\sigma_\xi^\star)$.
Fixing $\Delta S_{env}$ beyond its reversible bound cannot be done at an algorithmic level. While we leave evaluation of the true entropy flow $\Delta S_{env}$ to future work, we can demonstrate an example of this approach using an illustrative choice of the entropy flow: $\Delta S_{env}(\sigma_x,\sigma_\xi) = \Delta S_{env,Ex}(\sigma_x,\sigma_\xi) = \Delta S_{env,SGD}(\sigma_x,\sigma_\xi) = C + \alpha(\sigma_x^2 + \sigma_\xi^2)$, as shown in Fig.~\ref{fig:MMC}. 


\pagebreak
\FloatBarrier
