# Supplementary material for: The Entropy of Floating-Point Numbers
Source: arXiv:2605.11546 source file (2026-09-02)
Supplement: Supplementary file 7 [file prob_dist_z.tex]

\section{Computing the Probability Distribution of Z}\label{sec:compute_f_z}

\begin{lemma}
    \label{lem:compute_f_z}
    Let $\bX \sim \mathcal{N}(0, \sigx^2 I_n)$ and $\bXi \sim \mathcal{N}(0, \sigxi^2 I_n)$ be independent, with $n \in \mathbb{N}$, and define $Z = \frac{\bX^T\bXi}{\bX^T\bX}$. The probability density function of $Z$ is
\begin{align}
    f_Z(z) = \sqrt{\frac{1}{\pi\paren{\sigx^2}^n\sigxi^2}}\frac{\Gamma\paren{\frac{n+1}{2}}}{\Gamma\paren{\frac{n}{2}}}\paren{\frac{\sigx^2\sigxi^2}{\sigx^2z^2 + \sigxi^2}}^{\frac{n + 1}{2}}
\end{align}
which is the probability density function of a scaled Student's t-distributed random variable with $n$ degrees of freedom and a scale of $\frac{\sigxi}{\sigx\sqrt{n}}$ \cite{JohnsonNormanLloyd1994Cud}. 
\end{lemma}

\begin{proof}[Proof of Lemma~\ref{lem:compute_f_z}]
Recall that $Z = \frac{\xv^T\xiv}{\xtx}$. Using the law of total probability, we have
\begin{align}
    f_{Z}(z) &= \int f_{Z|\xv} (z|\xv)f_\xv(\xv)d\xv.
\end{align}
We see that $f_{Z|\xv} (z|\xv) \sim \gauss{0}{\frac{\sigxi^2}{\xv^T\xv}}$. Let $\xt \sim \gauss{0}{\frac{\sigx^2\sigxi^2}{\sigx^2z^2 + \sigxi^2}I}$. This means,
\begin{align}
    f_{Z}(z) &= \int \frac{\sqrt{\xtx}}{\sqrt{2\pi\sigxi^2}}e^{\frac{-(\xv^T\xv)z^2}{2\sigxi^2}}\paren{\frac{1}{\sqrt{2\pi\sigx^2}}}^ne^{-\frac{\xv^T\xv}{2\sigx^2}} d\xv\\
    &= \frac{1}{\sqrt{2\pi\paren{\sigx^2}^n\sigxi^2}}\paren{\frac{\sigx^2\sigxi^2}{\sigx^2z^2 + \sigxi^2}}^{\frac{n}{2}}\int \sqrt{\xtx}\paren{\frac{1}{\sqrt{2\pi}}}^n \paren{\frac{\paren{\sigx^2}^n\sigxi^2}{\sigx^2z^2 + \sigxi^2}}^{-\frac{n}{2}} e^{-\frac{\xtx}{2}\bracket{\frac{z^2}{\sigxi^2} + \frac{1}{\sigx^2}}}d\xv\\
    &= \frac{\E{\sqrt{\xttxt}}}{\sqrt{2\pi\paren{\sigx^2}^n\sigxi^2}}\paren{\frac{\sigx^2\sigxi^2}{\sigx^2z^2 + \sigxi^2}}^{\frac{n}{2}}.
\end{align}

Let $c \triangleq \frac{\sigx^2\sigxi^2}{\sigx^2z^2 + \sigxi^2}$ and let $\mathbf{g} \sim \mathcal{N}(0, I_n)$. We have $\E{\sqrt{\xttxt}} = \sqrt{c}\,\E{\sqrt{\mathbf{g}^T\mathbf{g}}} = \sqrt{2c}\frac{\Gamma\paren{\frac{n+1}{2}}}{\Gamma\paren{\frac{n}{2}}}$, where the last equality uses $\sqrt{\mathbf{g}^T\mathbf{g}} \sim \chi(n)$ \cite{JohnsonNormanLloyd1994Cud}. Therefore,
\begin{align}
    f_Z(z) &= \sqrt{\frac{1}{\pi\paren{\sigx^2}^n\sigxi^2}}\sqrt{\frac{\sigx^2\sigxi^2}{\sigx^2z^2 + \sigxi^2}}\frac{\Gamma\paren{\frac{n+1}{2}}}{\Gamma\paren{\frac{n}{2}}}\paren{\frac{\sigx^2\sigxi^2}{\sigx^2z^2 + \sigxi^2}}^{\frac{n}{2}}\\
    &= \sqrt{\frac{1}{\pi\paren{\sigx^2}^n\sigxi^2}}\frac{\Gamma\paren{\frac{n+1}{2}}}{\Gamma\paren{\frac{n}{2}}}\paren{\frac{\sigx^2\sigxi^2}{\sigx^2z^2 + \sigxi^2}}^{\frac{n + 1}{2}}\label{eq:f_z_appendix}
\end{align}
This distribution is depicted in Fig.~\ref{fig:z_fit} for varying values of $n$.
\end{proof}


\begin{figure}[htbp]
  \centering
  \begin{subfigure}{0.33\textwidth}
    \centering
    \includegraphics[width=\linewidth]{Exact/slope_fit_distribution_N=3.pdf}
    \caption{$n = 3$}
    \label{fig:z_fit_3}
  \end{subfigure}\hfill
  \begin{subfigure}{0.33\textwidth}
    \centering
    \includegraphics[width=\linewidth]{Exact/slope_fit_distribution_N=10.pdf}
    \caption{$n=10$}
    \label{fig:z_fit_10}
  \end{subfigure}\hfill
  \begin{subfigure}{0.33\textwidth}
    \centering
    \includegraphics[width=\linewidth]{Exact/slope_fit_distribution_N=30.pdf}
    \caption{$n=30$}
    \label{fig:z_fit_30}
  \end{subfigure}
  \caption{\textit{The probability density function} $f_Z(z)$, with $\sigx = \sigxi = 1$. As $n$ increases, the distribution becomes more peaked around $z = 0$. The simulation is of 50000 trials.} 
  \label{fig:z_fit}
\end{figure}

\FloatBarrier
\pagebreak
