# Supplementary material for: The Entropy of Floating-Point Numbers
Source: arXiv:2605.11546 source file (2026-09-02)
Supplement: Supplementary file 8 [file scaling_laws_app.tex]

\section{Derivations for Energy-cost Aware Scaling Laws}\label{sec:scaling_laws_app}

\subsubsection{Exact Formula}
Using the generalization error scaling for the exact linear regression formula in Eq.~\eqref{eq:exact_error}, we can solve a continuous relaxation of the optimization problem in Eq.~\eqref{eq:scaling_opt} where $\tilde n \in \R{}$. Let \begin{equation}\label{eq:u_ex}
u_{Ex}(\tilde n) \triangleq \rho_I\frac{\tilde n-2}{(\tilde n-1)\sigxi^2} - \rho_{J}\Delta E_{min}^{Ex}\paren{\tilde n}.
\end{equation}
 The optimization problem now becomes
\begin{align}
    \tilde n^\star &= \arg\max\limits_{\tilde n \geq 3} u_{Ex}(\tilde n) \text{, and } \nonumber\\
    n^\star &= \arg\max_{n\in\{\lfloor \tilde n^\star\rfloor,\lceil \tilde n^\star\rceil\}} u_{Ex}(n)\label{eq:nstar_ex}.
\end{align}
For simplicity, assume $|w| \gg \frac{\sigxi}{\sigx}$. Although the following method could be derived using the exact entropy calculations in Sections~\ref{sec:fpn}~and~\ref{sec:exact}, we will use $\tilde H_s(\Xfp, \Yfp)$ from Eq.~\eqref{eq:approx_joint_ent_SNR} and $\tilde H^w_s(\Wh_{fp}) = h(Z) + (p-1) -\log\bracket{\frac{|w|}{\sqrt{2}}}$ in this section for tractability. $h(Z)$ is computed in Lemma~\ref{lem:diff_ent_Ex}. Let $\psi^\prime(x) \triangleq \frac{d}{dx}\psi(x)$. Taking the derivative of $u$ with respect to $\tilde n$, we have
\begin{align}
    u^\prime_{Ex} (\tilde n) &= \frac{\rho_I}{\sigxi^2}\paren{\frac{1}{\tilde n-1}}^2\nonumber - \rho_J k_BT \ln[2] \paren{2\Ht^0_{s}(p) - \frac{1}{2}\log\bracket{ 1 + \frac{\sigma^2_x w^2}{\sigma_\xi^2}}- \frac{d}{d\tilde n}h(Z)}\label{eq:ddn_profit_ex},
\end{align}
where
\begin{align}
    \frac{d}{d\tilde n}h(Z) &= \log\bracket{e}\paren{\frac{\tilde n+1}{4} }\left(\psi^\prime\left(\frac{\tilde n+1}{2}\right)-\psi^\prime\left(\frac{\tilde n}{2}\right)\right).
\end{align}

It is not guaranteed that Eq.~\eqref{eq:ddn_profit_ex} will have a solution for all settings of parameters. It is recommended to solve the equation numerically using a root finder.\footnote{In our simulations, the profit function appears to be unimodal in $n$ which would justify the rounding procedure given in Eq.~\eqref{eq:nstar_ex}. We leave the proof of this unimodality for future work.} In Fig.~\ref{fig:ddn_profit_ex} we can see where $u^\prime_{Ex} (\tilde n)$ crosses zero for various setting of the price of energy $\rho_J$ and these zero crossings correspond to maximum values of the profit $u_{Ex}(n)$.

\subsubsection{Stochastic Gradient Descent}
\begin{figure}[bthp]
  \centering
  \begin{subfigure}{0.49\textwidth}
    \centering
    \includegraphics[width=\linewidth]{code/scaling/u_sgd_vary_eta.pdf}
    \caption{}
    \label{fig:profit_sgd_eta}
  \end{subfigure}
  \begin{subfigure}{0.49\textwidth}
    \centering
    \includegraphics[width=\linewidth]{code/scaling/u_sgd_vary_B.pdf}
    \caption{}
    \label{fig:profit_sgd_B}
  \end{subfigure}
  \begin{subfigure}{0.49\textwidth}
    \centering
    \hspace*{-0.35cm} 
    \includegraphics[width=\linewidth]{code/scaling/u_prime_sgd_vary_eta.pdf}
    \caption{}
    \label{fig:ddn_profit_sgd_eta}
  \end{subfigure}
  \begin{subfigure}{0.49\textwidth}
    \centering
    \hspace*{-0.35cm} 
    \includegraphics[width=\linewidth]{code/scaling/u_prime_sgd_vary_B.pdf}
    \caption{}
    \label{fig:ddn_profit_sgd_B}
  \end{subfigure}
  \caption{\textit{The effect of the learning rate and batch size on the optimal dataset size for stochastic gradient descent.} (\ref{fig:profit_sgd_eta}) shows $u_{SGD}(n)$ given in Eq.~\eqref{eq:u_sgd} for varying values of the learning rate $\eta$. Notice that smaller learning rates lead to larger optimal dataset sizes. (\ref{fig:ddn_profit_sgd_eta}) shows $u'_{SGD}(n)$ in Eq.~\eqref{eq:ddn_profit_sgd} for the different learning rates. (\ref{fig:profit_sgd_B}) shows $u_{SGD}(n)$ for various values of the batch size $B$. For the profit plots, the gold stars are the maximum values of the profit with respect to each algorithm's feasible set for each value of $\eta$ or $B$. (\ref{fig:ddn_profit_sgd_B}) shows $u'_{SGD}(n)$ for the different batch sizes. The vertical dotted lines show the point where each curve crosses zero. For all figures, $\sigxi^2 =\sigx^2 = 1$, $k_BT = 4\times 10^{-21}$, $w = 2$, $\wh_0 = 1$, $\rho_I = 10$, and $\rho_J = 5\times 10^{16}$. For the plots that vary $\eta$, $B=10$ and for the plots that vary $B$, $\eta = 0.05$.}
  \label{fig:scaling_laws_sgd_eta_B}
\end{figure}
For stochastic gradient descent, we can again take a continuous relaxation of the optimization problem in Eq.~\eqref{eq:scaling_opt}. Let 
\begin{equation}\label{eq:u_sgd}
u_{SGD}(\tilde n) \triangleq \rho_I\paren{\sigx^2\bracket{\frac{\eta\sigxi^2}{2B}\paren{1 -e^{-\frac{2\sigx^2 \eta \tilde n}{B}}} + \paren{\tilde \mu\paren{\frac{\tilde n}{B}} - w}^2} + \sigxi^2}^{-1} - \rho_J \Delta E_{min}^{SGD}\paren{\frac{\tilde n}{B}},
\end{equation} 
to obtain the optimization problem
\begin{align}
    \tilde n^\star &= \arg\max\limits_{\tilde n \geq B} u_{SGD}(\tilde n) \text{, and } \nonumber\\
    n^\star &= \arg\max_{n\in\{B\lfloor \tilde n^\star/B\rfloor,\, B\lceil \tilde n^\star/B\rceil\}} u_{SGD}(n)\label{eq:nstar_sgd},
\end{align}
where the rounding ensures $n^\star \in B\N{}$, since the total number of SGD training samples must satisfy $n = kB$ for integer $k$.
Under the assumptions that the learning rate $\eta$ is small enough that $|\tilde \mu(k)| \gg \sqrt{\frac{\eta\sigxi^2}{2B}}$ throughout the optimization domain, and that $k$ is large enough for the OU approximation Eq.~\eqref{eq:langevin} to track the true SGD dynamics (see Section~\ref{sec:nonstationarysgd}), we can use the approximate entropy $\Ht^{\tilde \mu(k)}_s(\Wh_{fp,k})$ given in Eq.~\eqref{eq:three_approxes}. Taking the derivative of $u_{SGD}$ with respect to $\tilde n$, we have
\begin{align}
    &u^\prime_{SGD} (\tilde n) = -\rho_I\frac{\eta  \sigx^4 e^{-\frac{2 \eta  \tilde n \sigx^2}{B}} \left(\eta  \sigxi ^2-2 B (w-\wh_0)^2\right)}{B^2\paren{\sigx^2\bracket{\frac{\eta\sigxi^2}{2B}\paren{1 -e^{-\frac{2\sigx^2 \eta \tilde n}{B}}} + \paren{\tilde \mu\paren{\frac{\tilde n}{B}} - w}^2} + \sigxi^2}^{2}} \nonumber\\
    &- \rho_J k_BT \ln[2] \Bigg(2\Ht^0_{s}(p) - \frac{1}{2}\log\bracket{ 1 + \frac{\sigma^2_x w^2}{\sigma_\xi^2}}+ \frac{\eta  \sigx^2  \left(w \left(1-e^{-\frac{\eta  \tilde n \sigx^2}{B}}\right)-\wh_0 \right)}{B \ln\bracket{2} \left(1 - e^{-\frac{2 \eta  \tilde n \sigx^2}{B}}\right) \left(w \left(e^{\frac{\eta  \tilde n \sigx^2}{B}}-1\right)+\wh_0\right)}\Bigg).\label{eq:ddn_profit_sgd}
\end{align}

Similar to the exact formula case, in Fig.~\ref{fig:ddn_profit_sgd} we plot $u^\prime_{SGD} (n)$ for various $\rho_J$ and show that its zero crossings correspond to maxima in  $u_{SGD} (n)$ in Fig.~\ref{fig:profit_sgd}. The optimal dataset size decreases as $\rho_J$ increases.




\pagebreak
\FloatBarrier
