# Supplementary material for: The Entropy of Floating-Point Numbers
Source: arXiv:2605.11546 source file (2026-09-02)
Supplement: Supplementary file 9 [file sgd_fit_quality.tex]

\section{SGD Fit Quality}

Here we review the fit quality of approximations introduced to obtain analytic expressions for the entropy of model parameters along stochastic gradient descent. Fig.~\ref{fig:assymp_fit} shows the asymptotic fit quality, while Fig.~\ref{fig:non_assymp_fit} shows the nonasymptotic fit quality.

\begin{figure}[htbp]
  \centering
    \centering
    \includegraphics[width=0.3\linewidth]{stationary/assymp_fit (1).pdf}
  \caption{\textit{Fit quality for asymptotic stochastic gradient descent.} Empirical investigation of the validity of the continuous Ornstein-Uhlenbeck process approximation with a simulation of $\hat w$ with $\eta = 0.01$, $\tau = 200$, $\sigma_x^2 = 1$, and $\sigma_\xi^2=1$, for 1000 trials. From top to bottom, the batch sizes are $B = \{1,5,25\}$ while $\tau = 200$, showing the approximation is already effective for these parameters at low $B$. }
  \label{fig:assymp_fit}
\end{figure}

\begin{figure}[htbp]
  \centering
  \begin{subfigure}{0.42\textwidth}
    \centering
    \includegraphics[width=\linewidth]{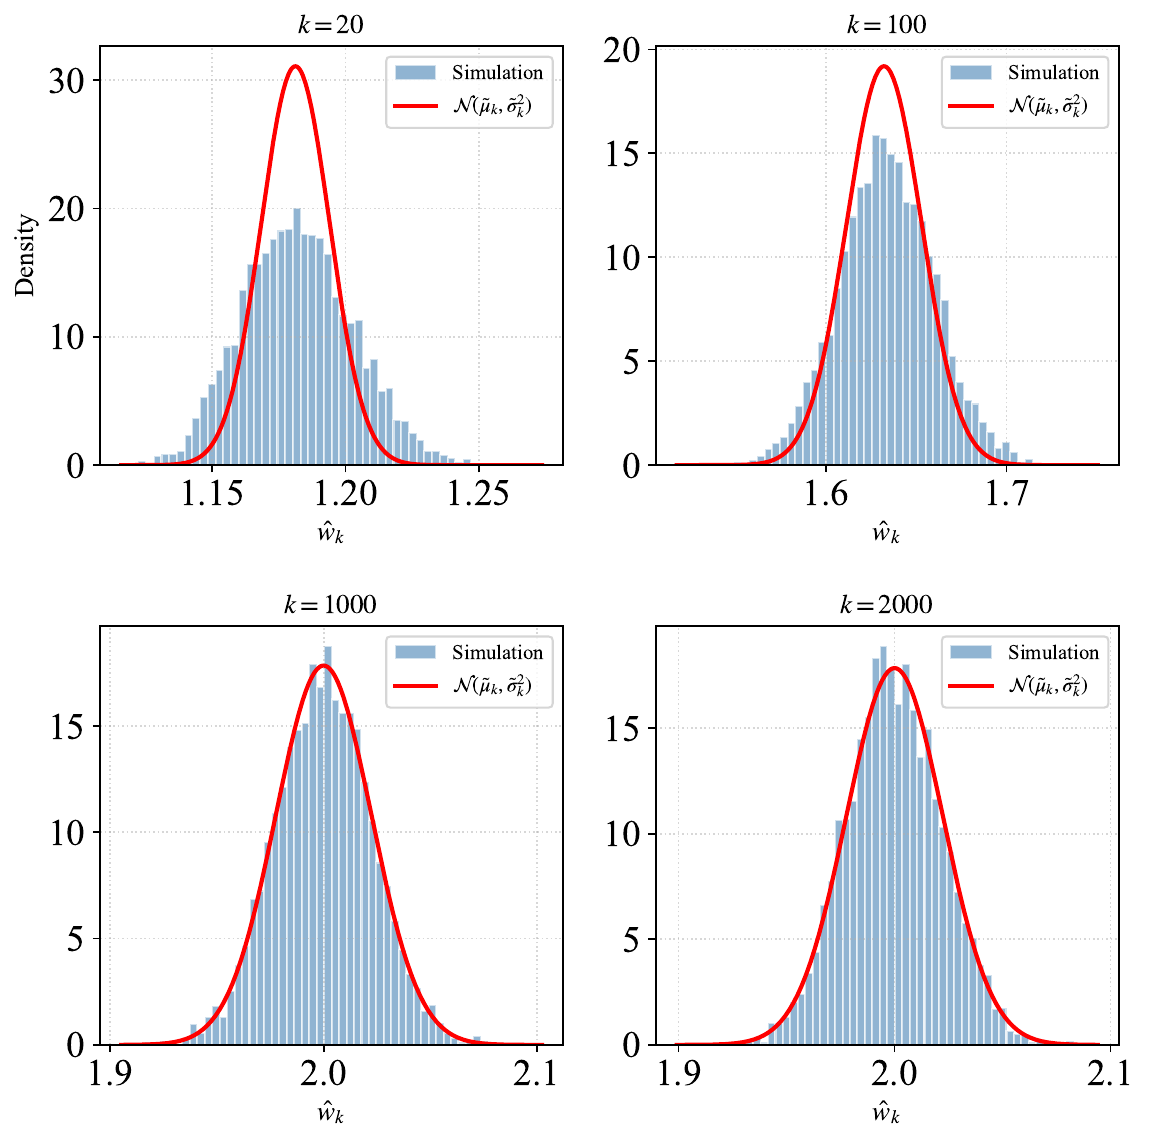}
    \caption{}
    \label{fig:non_assymp_fit}
  \end{subfigure}
  \begin{subfigure}{0.3\textwidth}
    \centering
    \includegraphics[width=\linewidth]{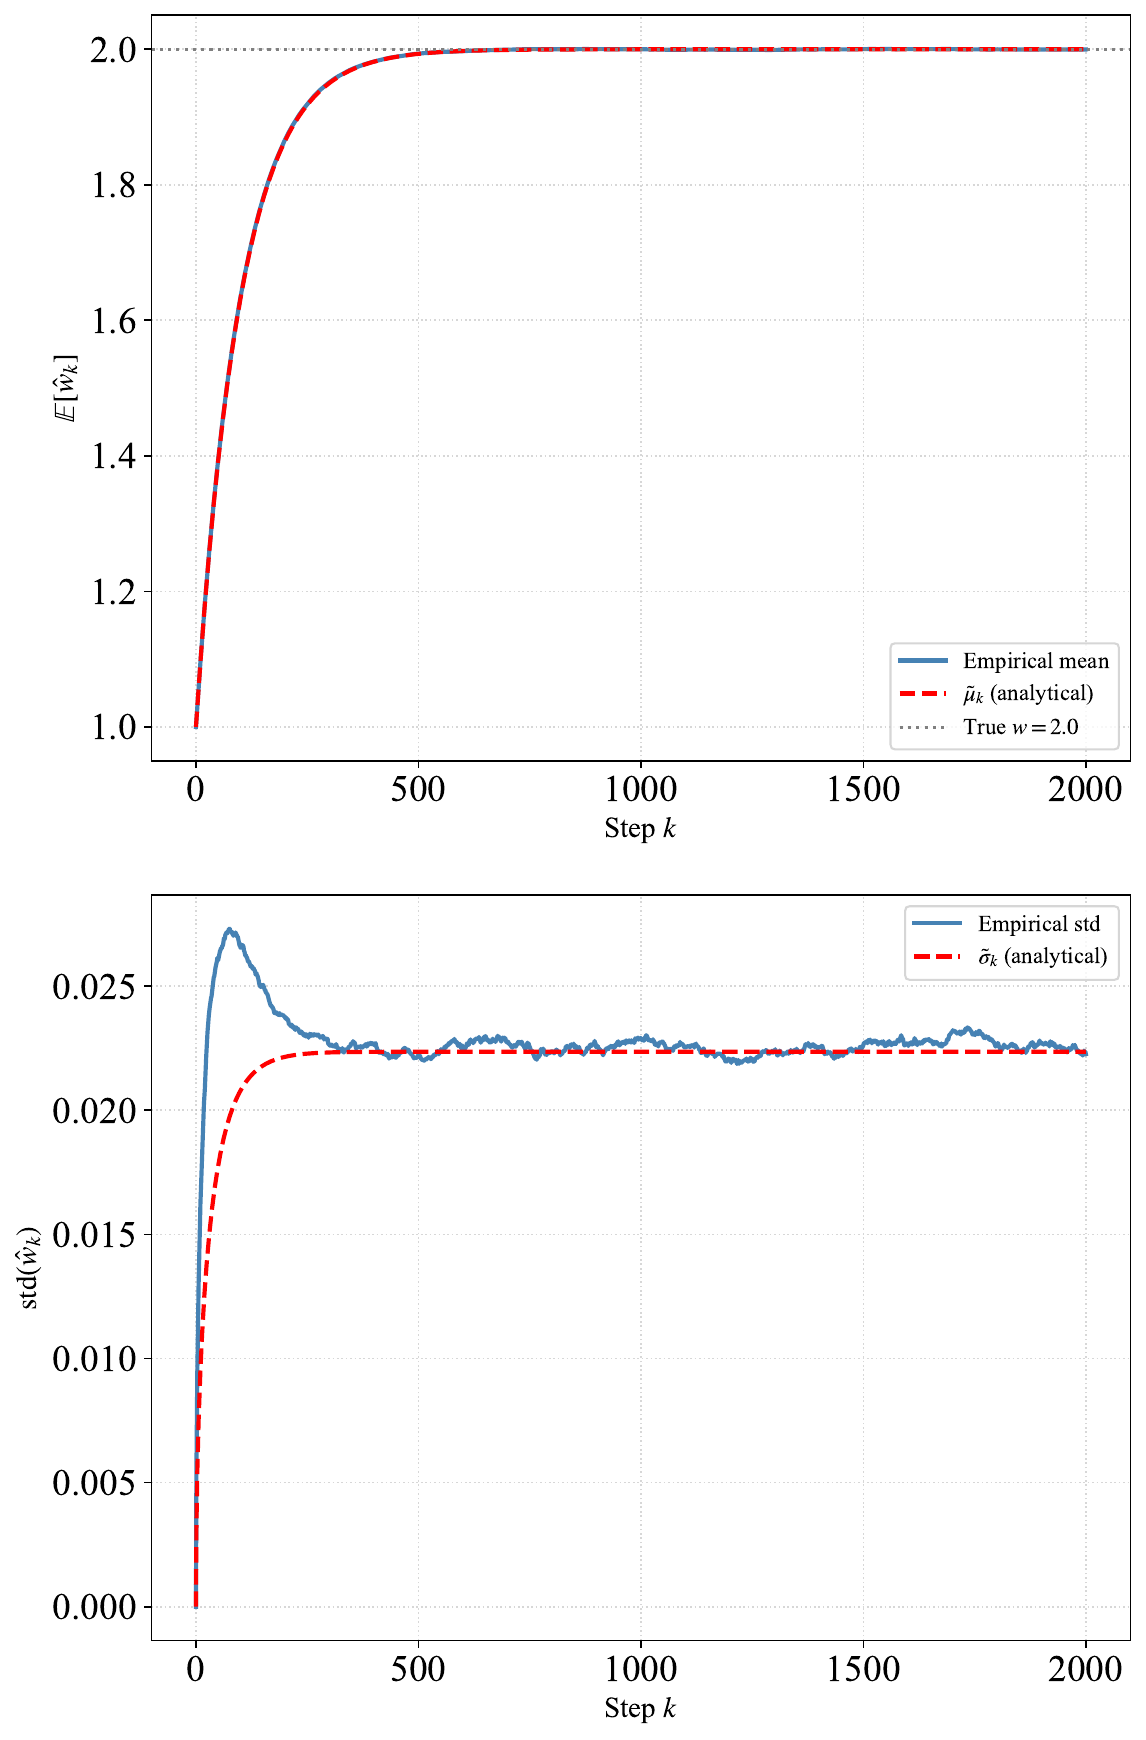}
    \caption{}
    \label{fig:mean_fit}
  \end{subfigure}
  \caption{\textit{SGD dynamics for zero-intercept simple linear regression.} (\ref{fig:non_assymp_fit}) SGD parameter $\hat w$ distribution at selected iterations, for 5000 separate trials of running SGD. $\sigx^2 = 1$, $\sigxi^2 = 1$, $\eta = 0.01$, $B = 10$. (\ref{fig:mean_fit}) Theoretical mean and standard deviation compared to the empirical mean and standard deviation as step number $k$ increases up to final value $k = \tau = 2000$.}
  \label{fig:sgd_w_2x2}
\end{figure}

\FloatBarrier
\pagebreak
